# Supplementary material for: Propagation of pop ups in kirigami shells
Source: arXiv:1905.00187 source file (2019-05-01)
Supplement: Supplementary file 1 [file manuscript_SI.pdf]

# Supplementary Information for

## Propagation of pop-ups in kirigami shells

**Ahmad Rafsanjani, Lishuai Jin, Bolei Deng and Katia Bertoldi**

**Corresponding Author: Katia Bertoldi**
**John A. Paulson School of Engineering and Applied Sciences**
**Harvard University, Cambridge, MA 02138, USA**
**E-mail: bertoldi@seas.harvard.edu**

### This PDF file includes:

Supplementary text
Figs. S1 to S25
Captions for Movies S1 to S9
References for SI reference citations

### Other supplementary materials for this manuscript include the following:

Movies S1 to S9

## Supporting Information Text

## 1. Fabrication

All kirigami structures investigated in this study are fabricated by laser cutting an array of cuts into polyester plastic sheets (Artus Corporation, NJ) with thickness $t \sim 76.2\,\mu$m, Young's modulus $E = 4.33$ GPa and Poisson's ratio $\nu = 0.4$. As shown in Fig. S1, the laser cutting process results in cuts with width $w_c \simeq 0.1$ mm.

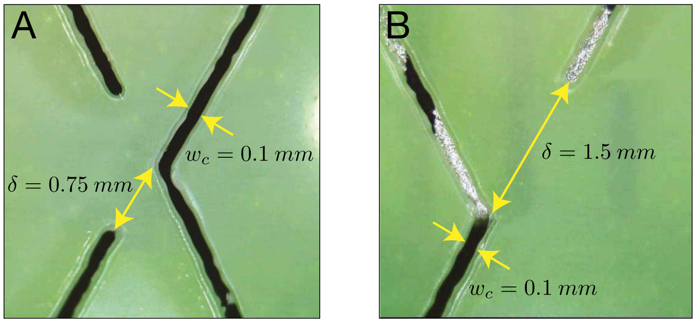


**Fig. S1.** Microscope image (Supereyes A005+ 5MP 500X) of a sheet laser cut to embed a triangular array of cuts with hinges of width (*A*) $\delta = 0.75$ mm and (*B*) $\delta = 1.50$ mm. We find that the laser cutting process results in cuts with width $w_c \simeq 0.1$ mm.

**A. Kirigami shells.** The cylindrical kirigami shells are then fabricated by rolling the laser cut kirigami sheets and attaching their two opposite edges to each other using a 0.07 mm thick double-sided adhesive sheet (23205-1009, Blick Art Materials, IL) (Figs. S2*A* and *B*). Note that a row of needles is used to ensure overlapping of the cuts located near the opposite edges and thus maintain the periodicity of the structure (Figs. S2*C* and *D*). Finally, two acrylic circular caps are glued to the both ends of the cylinder (Figs. S2*E* and *F*) and two screws are bolted at the center of the caps to facilitate attaching the samples to the tensile testing machine (see Supporting Movie S1).

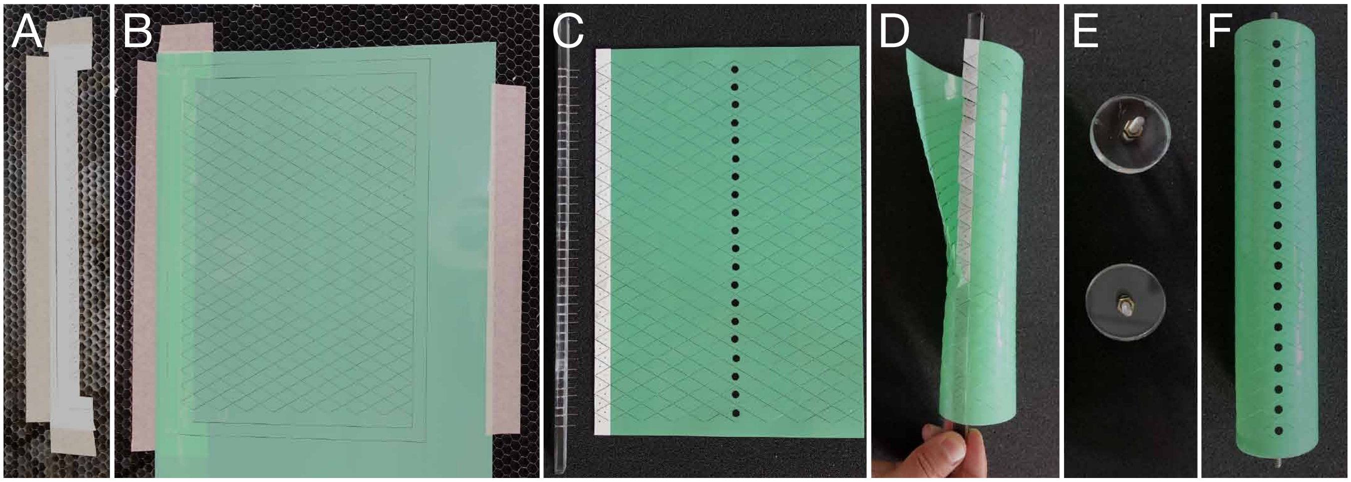


**Fig. S2.** Fabrication of a kirigami shell: (*A*) the double-sided adhesive is laser cut into the desired shape; (*B*) the polyester sheet is attached to the adhesive layer and the kirigami pattern is laser cut; (*C*) very thin adhesive black markers are attached to the sheet to track the deformation during testing; (*D*) the two edges of the sheet are attached together using needles to facilitate alignment; (*E*) two bolted acrylic caps are laser cut; (*F*) the caps are glued to the cylinder ends.

In this study three different kirigami patterns are considered:

- *Triangular pattern:* In this pattern, the cuts are arranged on a triangular lattice with lattice constants $l$ and $\gamma = \pi/3$ (6). The unit cell considered in this study is highlighted in gray in Fig. S3*A*. It consists of a rectangular domain with width $L = 2l\cos\pi/6$ and height $H = 2l\sin\pi/6$ with embedded four cuts of length $l - \delta$ separated by hinges of width $\delta$.

- *Linear pattern:* This pattern, which has been considered in several studies (2–4), comprises an array of staggered linear cuts of length $l - \delta$ separated in horizontal direction by hinges of width $\delta$ and in vertical direction by $l/8$. The unit cell considered in this study with width $L = l$ and height $H = l/4$ is highlighted in gray in Fig. S3*B*.

- *Orthogonal pattern:* This pattern consists of a square array of mutually orthogonal cuts (5). This perforation pattern introduces a network of square domains of edge $l$ separated by hinges of width $\delta$. The unit cell considered in this study with width $L = 2l$ and height $H = 2l$ is highlighted in gray in Fig. S3*C*.

Throughout the study, we fix the size of the unit cells ($L$ and $H$) for each pattern. In particular, for the triangular pattern we choose $l = 12$ mm and $\gamma = \pi/3$, resulting in $L = 20.8$ mm and $H = 12$ mm, for the linear pattern $l = L = 12$ mm and $H = 3$ mm, and for the orthogonal pattern we choose $l = 6$ mm, leading to $L = H = 12$ mm. As a result, the number of units along the circumference $n$ uniquely determine the size of cylinder. Specifically, the two acrylic caps that we glue at its two ends have radius $r = nL/(2\pi)$. However, it is important to note that, because of the cuts, the radius of the kirigami cylinder is not constant and varies both around the circumferential and axial directions.

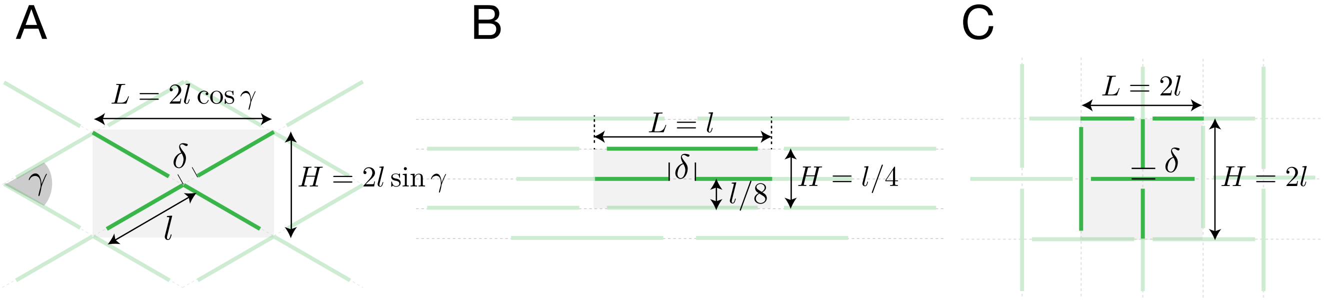


**Fig. S3.** Three different kirigami patterns are considered in this study: (*A*) triangular pattern with $\gamma = \pi/3$, (*B*) linear pattern and (*C*) orthogonal pattern. The unit cell of each pattern is shaded.

## 2. Experiments

The quasi-static uniaxial tensile response of the kirigami sheets and kirigami cylinders is probed using an uniaxial testing machine (Instron 5566) equipped with a 10N load cell. All tests are conducted under displacement control at a rate of 0.5 mm/s. During these tests we record the motion of the structures using a high-resolution camera (SONY RX100V) at a frame rate of 30 fps and extract their local deformation using an open-source digital image correlation and tracking package (7). We track the position of 20 markers uniformly placed on a vertical line (see Fig. S4*A*) and use these data to characterize both the applied deformation and the evolution of the local deformation as a function of the applied strain. Specifically, the applied strain $\bar{\varepsilon}$ is obtained as

$$\bar{\varepsilon} = \frac{z_q - z_p}{Z_q - Z_p} - 1, \qquad \text{[S1]}$$

where $z_i$ and $Z_i$ denote the position of the $i$-th marker in the deformed and undeformed configuration, respectively. Note that, to minimize boundary effects, in Eq. S1 we choose $(p, q) = (3, 18)$, $(5, 55)$ and $(1, 30)$ for structures with triangular, linear and orthogonal patterns, respectively. As for the local deformation, focusing on the $i$-th row of cuts the normal strain in longitudinal direction is calculated as

$$\varepsilon_i = \frac{z_{i+1} - z_i}{Z_{i+1} - Z_i} - 1. \qquad \text{[S2]}$$

Additional experimental results are provided in Figs. S4- S6.

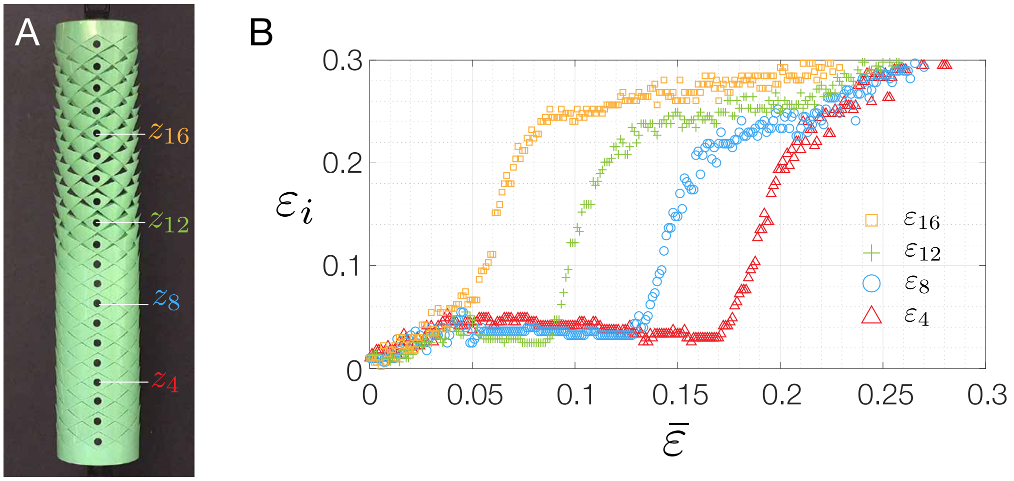


**Fig. S4.** Local strain distribution in a kirigami shell with triangular cuts: (*A*) Kirigami cylinder with $n = 8$ and $\delta/l = 0.0625$ (with $l = 12$ mm). (**B**) Evolution of $\varepsilon_i$ (with $i$ =4, 8, 12 and 16) as a function of the the applied strain $\bar{\varepsilon}$.

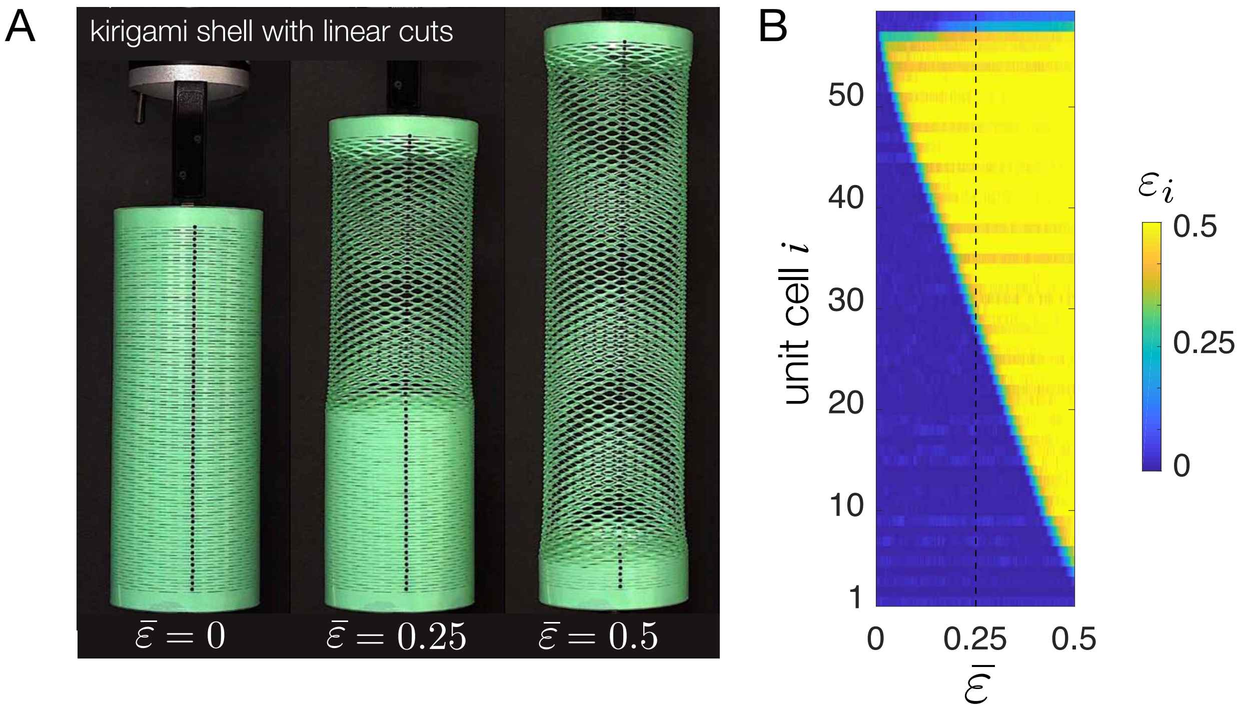


**Fig. S5.** (*A*) Snapshots of kirigami shells with linear cuts which are characterized by $\delta/l = 0.2$ (with $l = 12$ mm) and $n = 20$ at $\bar{\varepsilon} = 0, 0.25$ and $0.5$. The snapshots clearly indicate that instability propagation in this kirigami shells is characterized by a very sharp and narrow front. (*B*) Contour map of local strains $\varepsilon_i$ as a function applied strain $\bar{\varepsilon}$ and unit cell number $i$.

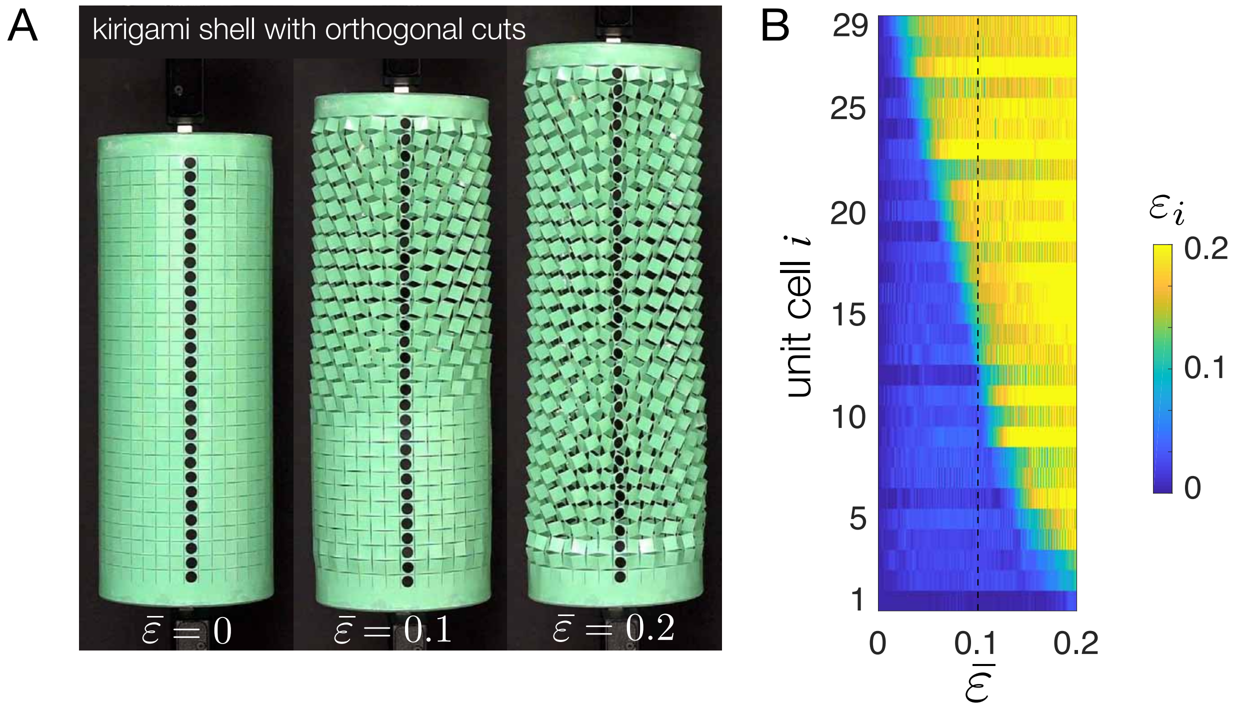


**Fig. S6.** (*A*) Snapshots of kirigami shells with orthogonal cuts which are characterized by $\delta/l = 0.08$ (with $l = 6$ mm) and $n = 20$ at $\bar{\varepsilon} = 0, 0.1$ and $0.2$. The snapshots clearly indicate that instability propagation in this kirigami shells is characterized by a wider front compared to that found for the shell with linear pattern considered in Fig. S5. (*B*) Contour map of local strains $\varepsilon_i$ as a function applied strain $\bar{\varepsilon}$ and unit cell number $i$. The orthogonal pattern has a wider front compared to linear pattern.

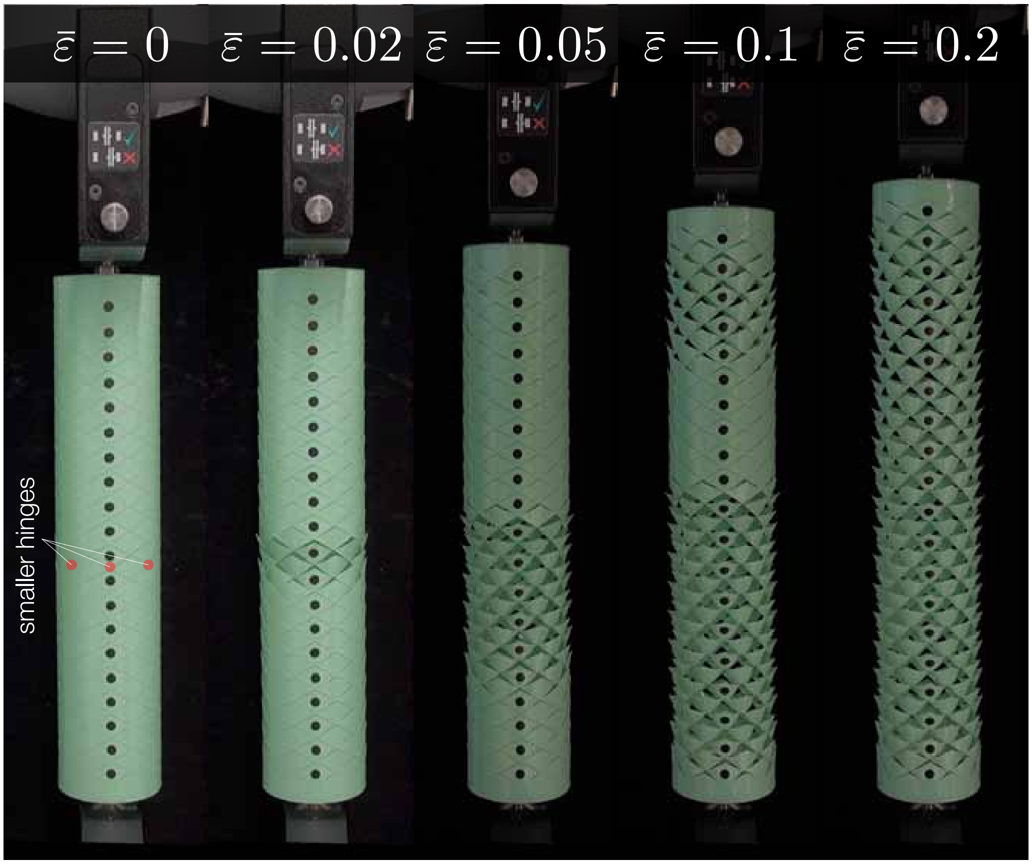


**Fig. S7.** Effect of imperfection. Snapshots of a kirigami shells with triangular cuts which is characterized by $\delta/l = 0.125$ (with $l = 12$ mm) and $n = 8$ at $\bar{\varepsilon} = 0,\ 0.02,$ 0.05, 0.1 and $0.2$. An imperfection is introduced in the middle of the shell by decreasing the width of one row of hinges (highlighted in red) to $\delta/l = 0.0625$. We find that the pop-ups initiate near the imperfection and propagate downwards until it reaches the bottom boundary. Further stretching triggers pop-ups from the top boundary and they continue propagating to reach the region which is already popped up. Finally the shell stretches uniformly (see Movie S9).

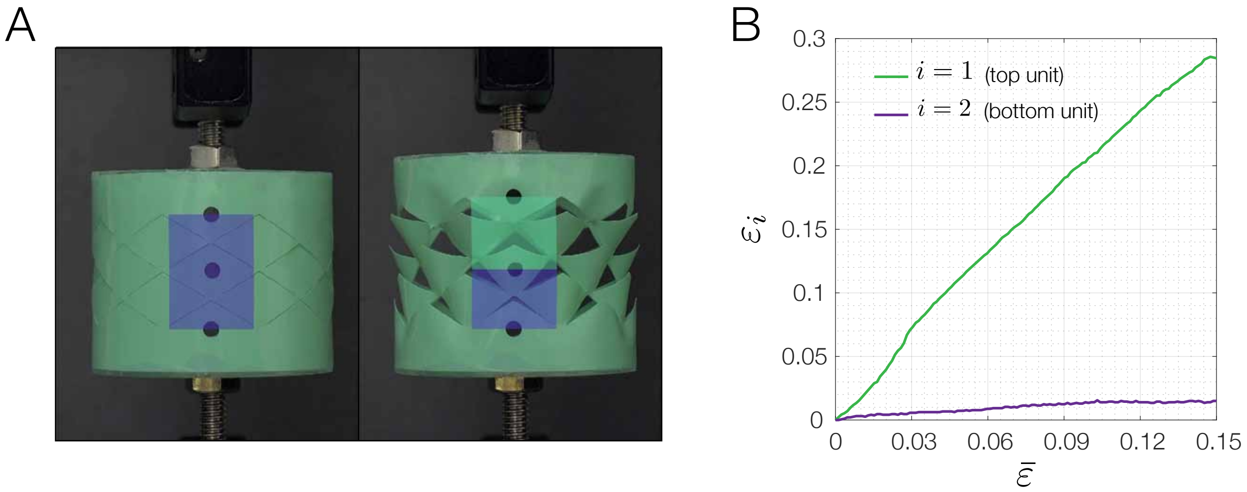


**Fig. S8.** Compliance of the boundaries. (*A*) In our experiments the pop-up process always starts from the top end (i.e. the end to which all triangular features are pointing), suggesting that the two ends of the kirigami shells introduce imperfections of different magnitude. To verify this, we test a kirigami shell with $n = 8$ and $\delta/l = 0.0625$ and monitor the local strain of the unit cells. (*B*) Evolution of $\varepsilon_1$ (i.e. the strain of the unit cell next to the top edge) and $\varepsilon_2$ (i.e. the strain of the unit cell next to the bottom edge) as a function of the applied deformation $\bar{\varepsilon}$. We find that because of the asymmetry in geometry the unit cell next to the upper boundary is much more compliant - an observation that fully explains the initiation of the pop-ups from the top boundary.

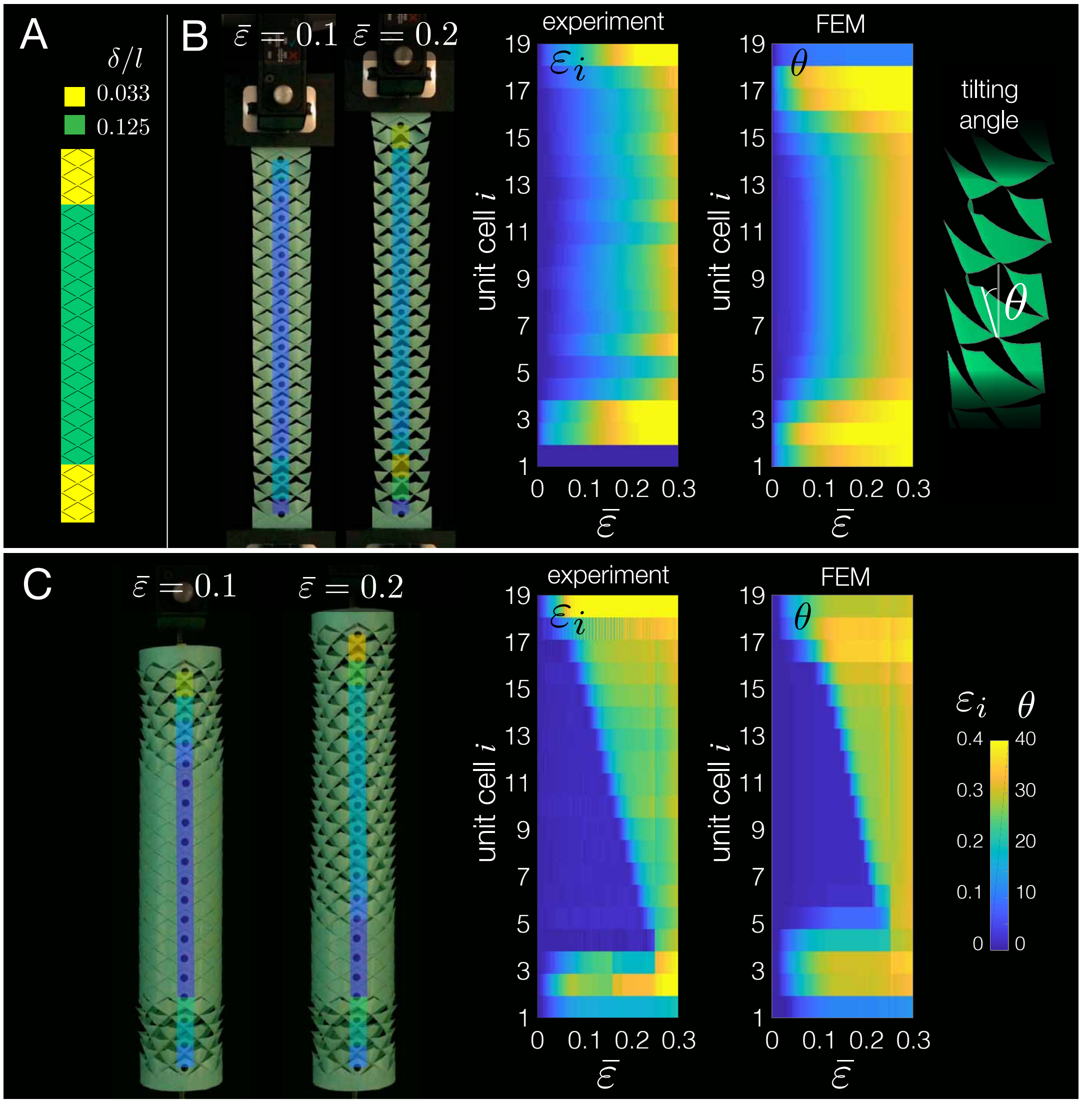


**Fig. S9.** (*A*) Schematic of our patterned kirigami surface. The triangular cuts are separated by ligaments with widths $\delta/l = 0.125$ in the central part (green region) and $\delta/l = 0.033$ near the two ends (yellow region). (*B*)-(*C*) Response of the patterned (*B*) kirigami sheet and (*C*) kirigami shell. The contour maps show the evolution of local strains $\varepsilon_i$ and tilting angles $\theta_i$ as a function of the applied deformation. Note that the local strains $\varepsilon_i$ are extracted from the experimental images, while $\theta_i$ are obtained from FE simulations conducted on super-cells.

## 3. Kirigami-skinned crawlers

In this study we also use the kirigami cylindrical shells as smart skins to enhance the crawling efficiency of a linear actuator. Specifically, the kirigami-skinned crawlers tested in this study comprise a 30 mL plastic syringe as linear actuator covered with a kirigami shell with triangular cuts (see Fig. S10A). The two ends of the plastic syringe are connected to two acrylic circular caps, that in turn are glued to the ends of the kirigami shell. A flexible tube passing through the rear cap then connects the actuator to a syringe pump which is programmed to cyclically inflate/deflate the plastic syringe. This results in an extension of the actuator of about 54 mm at 2.74 mm/s. Note that we choose a rigid linear actuator - as opposed to soft actuator used in our previous study (6) - to exclusively investigate the behavior of the kirigami skin. However, a fully soft crawler can be easily realized by simply replacing the plastic syringe with a soft actuator.

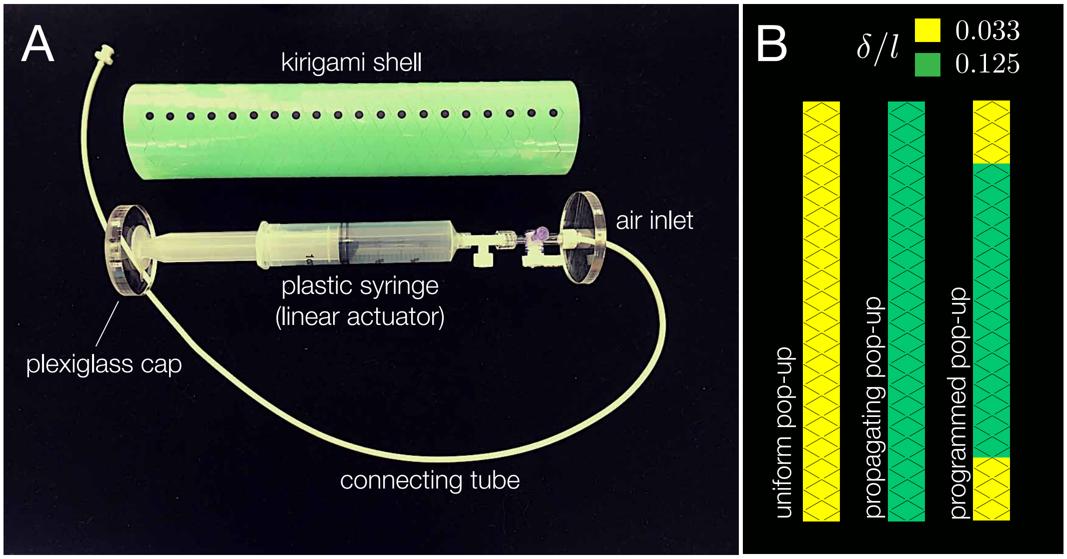


**Fig. S10.** (*A*) Components of the considered kirigami-skinned crawler. (*B*) Schematics of the three kirigami skins.

We consider three different kirigami skins, all comprising $8 \times 20$ triangular cuts with $l = 12$ mm and $\gamma = \pi/3$ (Fig. S10B):

- *Kirigami skin with uniform pop-up* with $\delta/l = 0.033$;
- *Kirigami skin with propagating pop-up* with $\delta/l = 0.125$;
- *Kirigami skin with programmed pop-up* with $\delta/l = 0.125$ for the central units and $\delta/l = 0.033$ for the first three units at the two ends.

To test the ability of the three crawlers to advance upon inflation and deflation of the syringe, we place them on the inner surface of an acrylic tube (with diameter of 65 mm) covered with a textile to increase friction. We find that for all three crawlers the elongation of the syringe triggers the pop-pop of the triangular scales, which in turn induces anisotropic frictional properties and enables our simple machines to move forward (6). However, since the anchorage to the ground is not perfect, there is always some backslide movement and not all the elongation induced by the syringe translates into advancement of the crawler (6). Remarkably, by comparing the performance of our three crawlers we find that the programmed pop-up achieved in our patterned shell enhances

the anchorage of the crawler to the substrate at two ends and significantly reduces the backslide (see Fig. S11B). As a result, the patterned crawler, which benefits from coexistence of popped and unpopped regions at desired locations, proceeds about twice faster than the other two.

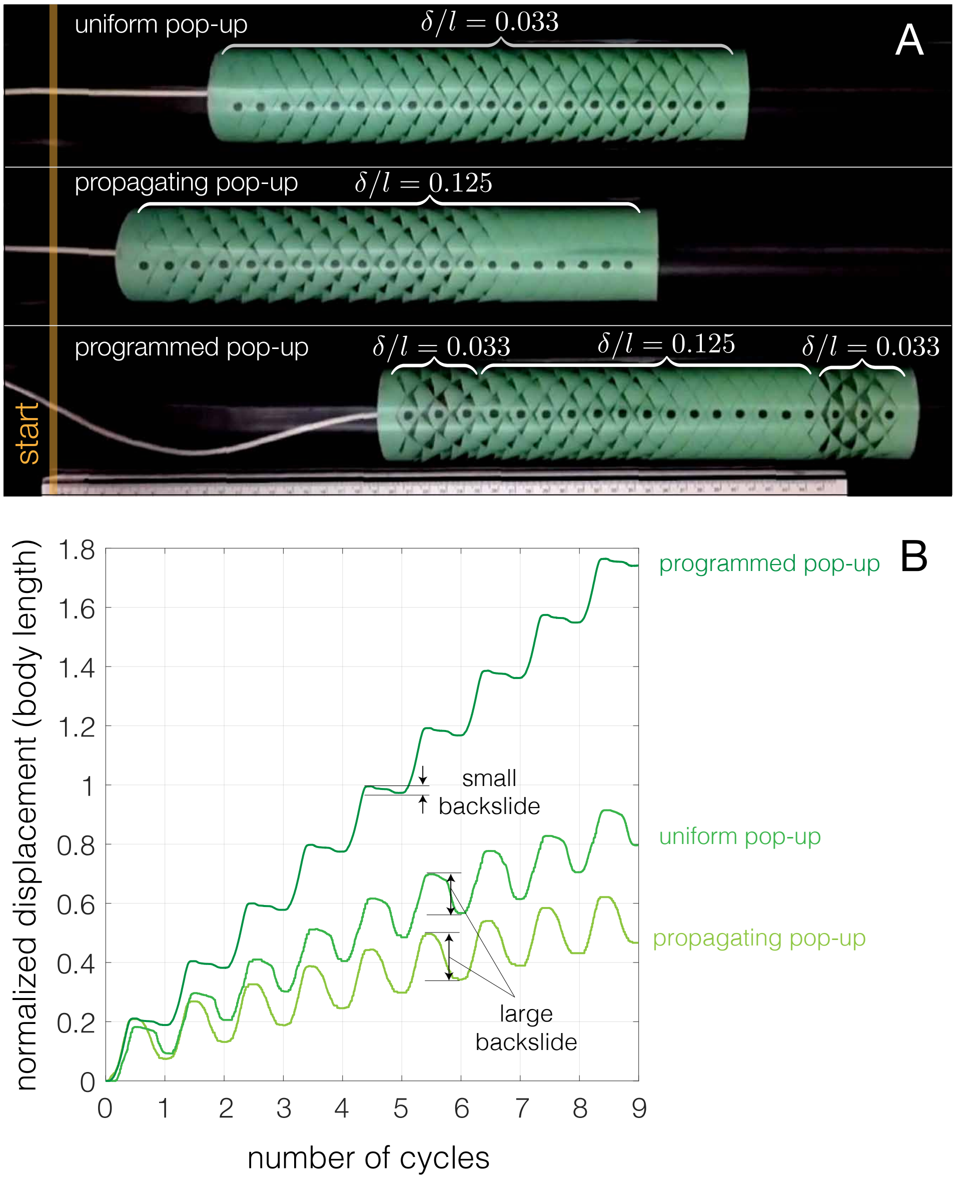


**Fig. S11.** (*A*) Snapshots of our kirigami-skinned crawlers with triangular cuts characterized by $\delta/l = 0.033$ (uniform pop-up), $\delta/l = 0.125$ and $\delta/l = 0.125$ for the central units and $\delta/l = 0.033$ for first three units at two ends (programmed pop-up). (*B*) Displacement of three crawlers normalized by their undeformed active body length (i.e. $NH$) as a function of the number of inflation/deflation cycles.

## 4. Modeling

To get a better understanding of the response of the considered kirigami structures, we investigate their behavior both numerically and analytically. First, we conduct Finite Element (FE) simulations on both unit cells and super-cells. Second, informed by these analyses, we establish an analytical model that predicts the stress required to trigger a propagative instability as well as the strain distribution within the structure during the propagation of the pop-ups.

**A. Finite Element Simulations.** To investigate the response of the kirigami structures under uniaxial stretch, we perform Finite Element (FE) Analyses using the commercial package ABAQUS 6.14/Standard (1). In all our analyses we discretize the sheets using four-node general-purpose shell elements with reduced integration and hourglass control (S4R element type) and, guided by our experiments (see Fig. S1) model the cuts as elongated rectangular voids with width of 0.1 mm. Since plasticity has little effect on the observed phenomena, the material behavior of the plastic sheets is captured using a linear elastic material model (with $E = 4.33$ GPa and $\nu = 0.4$). The response of the kirigami structures is then simulated conducting non-linear static simulations (`*STATIC` module in ABAQUS). Due to the existence of local buckling during the deformation, to facilitate convergence we also add volume-proportional damping to the model (using the option `STABILIZE` in ABAQUS) and set the dissipated energy fraction equal to 5e-4 and the maximum ratio of stabilization to strain energy equal to 0.05. To reduce the computational cost and make sure the response of the system is not dominated by boundary effects, we conduct analysis on both unit cells and super-cells comprising $N \times 1$ unit cells. For the unit cells, we apply periodic boundary conditions to all four edged, whereas for the super-cells we apply periodic boundary conditions only to the left and right ones.

In the following we provide details on the simulations we conduct to investigate the response of $(i)$ flat, $(ii)$ rolled and $(iii)$ curved kirigami sheets.

***Flat kirigami sheets.*** The simulations conducted to investigate the response of flat kirigami sheets consist of two steps.

*Step 1:* we apply a small displacement (with amplitude $0.1t$) normal to the sheet either to the tip of the cuts (in case of the triangular patterns) or to the middle of the cuts (in case of the linear and orthogonal patterns). In this way we introduce a small imperfection into the mesh to guide the post-buckling analysis. Note that to facilitate convergence during this step no traction and displacement are applied to the nodes lying on the external edges of the models.

*Step 2:* We apply a strain $\varepsilon$ to axially stretch the periodic cells. To simulate this on the unit cells, we apply periodic boundary conditions on all four edges. Specifically, we subject the unit cells to a macroscopic deformation

$$\overline{\mathbf{H}} = \varepsilon_{xx}\mathbf{e}_x \otimes \mathbf{e}_x + \varepsilon\, \mathbf{e}_z \otimes \mathbf{e}_z, \tag{S3}$$

by imposing the following periodic boundary conditions on all cell boundaries

$$\begin{aligned} &u_\alpha^{A_i} - u_\alpha^{B_i} = \overline{H}(X_\beta^{A_i} - X_\beta^{B_i}), \\ &\theta_\alpha^{A_i} = \theta_\alpha^{B_i} \quad i = 1, 2, ....N \end{aligned} \tag{S4}$$

where $u_\alpha^{A_i}$, $u_\alpha^{B_i}$, $\theta_\alpha^{A_i}$ and $\theta_\alpha^{B_i}$ ($\alpha = x$, $y$ and $z$) are the displacements and rotations of points periodically located on the boundary of the unit cell, $X_\beta^{A_i}$ and $X_\beta^{B_i}$ are their initial coordinates and $N$ denotes the number of pairs of nodes periodically located on the boundary of the unit cell. Moreover, $\varepsilon_{xx}$ is the stretch in transverse direction that is determined from $\sigma_{xx} = 0$. Note that the components of $\overline{\mathbf{H}}$ can be conveniently prescribed within the finite element framework using a set of virtual nodes.

The corresponding macroscopic first Piola-Kirchhoff stress $\overline{\mathbf{P}}$ is then obtained through virtual work considerations (11).

As for the super-cells, they are subjected to uniaxial tension by fixing all nodes on their top surfaces in $x$ and $y$ directions, while uniformly displacing them in $z$-direction. The applied nominal strain, $\varepsilon$, is then obtained as the ratio between the applied axial displacement and the initial length of the model. Moreover, the corresponding nominal stress, $S$, is calculated by dividing the total reaction force on the top edge by the undeformed cross-sectional area of the sample, $A = Lt$.

***Rolled kirigami sheets.*** The simulations conducted to investigate the response of rolled kirigami sheets also consist of two steps. Note that the periodic boundary conditions derived below are validated by comparison with analytical expressions for the deformation of a homogeneous (i.e. without cuts) sheet.

*Step 1:* We transform the flat model to a cylindrical one. We start with a flat unit cell with length $L$ and height $H$ (see Fig. S12) and roll it into a sector of a cylinder. At this point it is important to note that, because of the cuts, the radius of the kirigami cylinder is not constant and varies both around circumference and along the axial direction. To determine the boundary conditions required to roll a flat periodic cell into a cylindrical one, we assume that the flat cell is located at a distance $y_0$ from the center of the cylinder and symmetrically positioned with respect to the $y$ axis. Under these assumptions, we find that it can be rolled into a cylindrical shape when its *left* and the *right* edges are subjected to (see Fig. S12)

- a rotation with respect to the $z$-axis
$$\theta_z = \pm\frac{\pi}{n}, \qquad \text{[S5]}$$
- displacements in circumferential and radial direction that satisfy
$$y_0^2 + \frac{L^2}{4} = (\rho\cos\delta\phi + u_\rho)^2, \quad \sin\delta\phi = \frac{u_\phi}{\rho} \qquad \text{[S6]}$$

where $\rho$ and $\phi$ are respectively the radial and angular coordinates of the nodes periodically located on the edges and $\delta\phi = \pi/n - \arctan L/(2y_0)$. Guided by Eqs. S5 and S6, we then apply the following

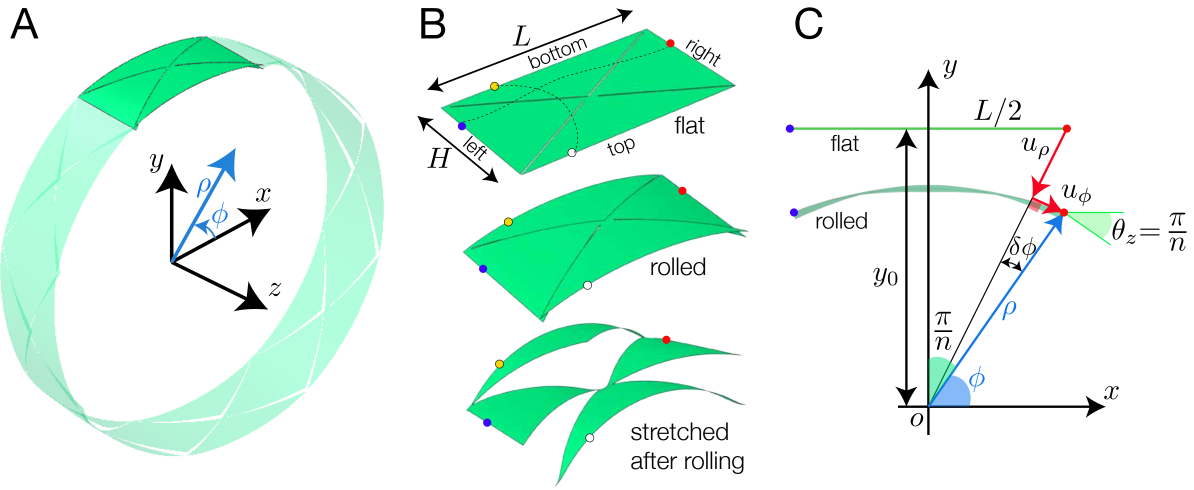


**Fig. S12.** (a) Schematic highlighting the coordinate system; (b) In our simulations, we start with a flat unit cell, we then roll it into a sector of a cylinder and finally stretch it. (c) Schematic highlighting the conditions that we use to roll the unit cell.

boundary conditions to the nodes periodically located on the left and right edges of the initially flat periodic cell

$$
\begin{aligned}
u_\rho^{R_i} &= u_\rho^{L_i},\\
u_\phi^{R_i} &= -\left(\sqrt{y_0^2 + L^2/4} - u_\rho^R\right)\tan\delta\phi,\\
u_\phi^{L_i} &= \left(\sqrt{y_0^2 + L^2/4} - u_\rho^L\right)\tan\delta\phi,\\
u_z^{R_i} &= u_z^{L_i},\\
\theta_\rho^{L_i} &= -\theta_\rho^{R_i},\\
\theta_\phi^{L_i} &= \theta_\phi^{R_i},\\
\theta_z^{L_i} - \theta_z^{R_i} &= \frac{2\pi}{n}, \quad i = 1, 2, ....N
\end{aligned}
\tag{S7}
$$

where $u_\alpha^j$ and $\theta_\alpha^j$ ($\alpha = \rho$, $\phi$, $z$ and $j = L_i$, $R_i$) are respectively the displacement and rotational degrees of freedom in the radial ($\rho$), circumferential ($\phi$) and axial ($z$) directions of the $i$-th pair of nodes periodically located on the *right* (R) and *left* (L) edges of the unit cell.

As for the top and bottom edges, we let them to be free, so that, as observed when fabricating our kirigami cylinders, the periodic cell can axially contract as it is rolled. To achieve this on the unit cells, we use Eqs. S4 with

$$\overline{\mathbf{H}} = \varepsilon_{zz}\mathbf{e}_z \otimes \mathbf{e}_z \tag{S8}$$

and determine $\varepsilon_{zz}$ by imposing $\sigma_{zz} = 0$.

*Step 2:* We apply a strain $\varepsilon$ to axially stretch the periodic cells. To simulate this on the unit cells, we keep active the boundary conditions defined by Eqs. S7 on the left and right edges, while on the top and bottom edges we still use Eqs. S4, but with

$$\overline{\mathbf{H}} = \varepsilon\, \mathbf{e}_z \otimes \mathbf{e}_z. \tag{S9}$$

Finally, for super-cells with $n_z \times 1$ units, we impose Eq. S7 on their left and right edges, fix all the degrees of freedom of the nodes on the bottom edge (i.e. we set $u_z^B = u_\phi^B = u_\rho^B = \theta_\phi^B = \theta_\rho^B = \theta_z^B = 0$) and set $u_z^T = \varepsilon n_z H$ and $\theta_\rho^T = \theta_\phi^T = 0$, while leaving $u_\rho^T$, $u_\phi^T$ and $\theta_z^T$ free.

**Validation of the periodic boundary conditions used to simulate the response of rolled kirigami sheets**
To confirm the validity of the proposed approach to simulate the response of rolled cylinders, we compare FE results (obtained by using Eqs. S7 and Eqs. S4 with Eq. S8 and Eq. S9) against analytical solutions for a homogeneous sheet which is first rolled into a cylinder and then stretched (Fig. S13*B*). To derive such analytical solution, we start by noting that, when the bending radius $r$ and the width of the sheet $L$ are much larger than the sheet thickness $t$, during the rolling/bending process: ($i$) the cross section of the sheet remains planar; ($ii$) the neutral layer coincides with the mid-plane; ($iii$) there is no stress in radial direction (i.e. $\sigma_y = 0$); and ($iv$) there is no deformation in axial direction (i.e. $\varepsilon_z = 0$). Under these assumptions, the Hook's Law reads

$$\sigma_x = \frac{E\varepsilon_x}{1-\nu^2}. \tag{S10}$$

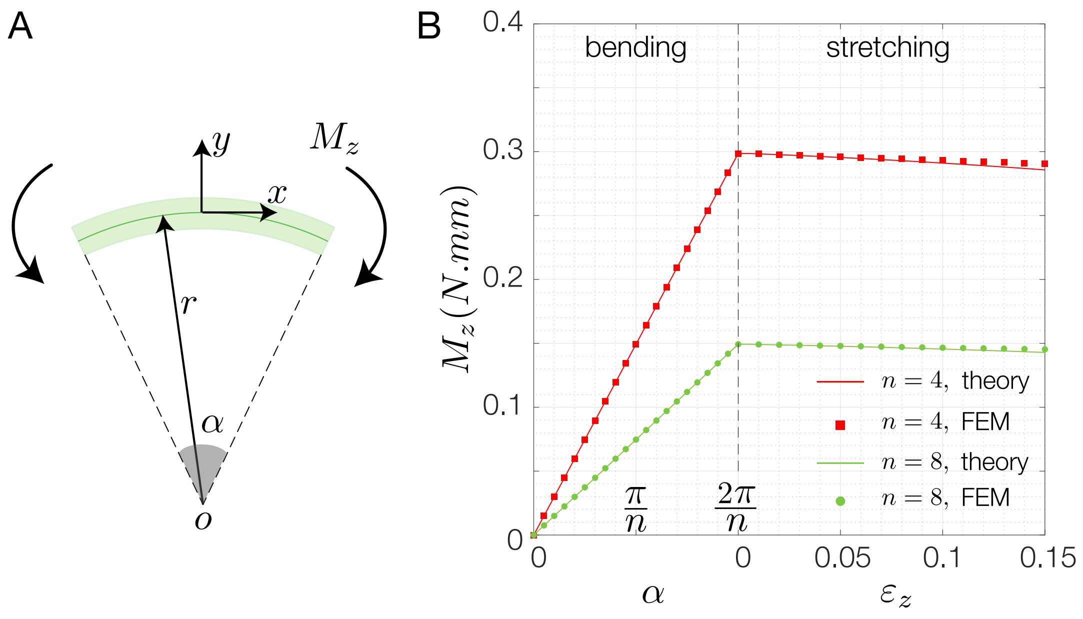


**Fig. S13.** Validation of the periodic boundary conditions by comparing analytical solutions [Eq. S12] and FE simulations for a solid sheet that is first rolled into a (portion of) a cylinder and then stretched. (*A*) Schematic of the unit cell. (*B*) Comparison between FE and analytical results for $n$= 4 and 8.

where $\varepsilon_x = y/r$ is the circumferential strain, $r = L/\alpha$ being the radius of the cylinder. It follows that the bending moment $M_z^{bending}$ required to bend the flat cell into a curved one is given by

$$M_z^{bending} = \int_{-t/2}^{t/2} \sigma_x H y dy = \frac{EHt^3\alpha}{12L\,(1-\nu^2)}. \quad \text{[S11]}$$

As for the stretching process, because of the Poisson's effect, we expect the sheet to shrink circumferentially, so that

$$\varepsilon_x = \frac{y}{r} - \nu\varepsilon_z, \qquad \varepsilon_y = -\nu\varepsilon_z \quad \text{[S12]}$$

$\varepsilon_z$ denoting the applied axial stretch. Moreover, during stretching $\alpha = 2\pi/n$ and $r = nL/2\pi$ ($n$ being the number of unit cell along the circumference). Consequently, the bending moment during the stretching process reads:

$$M_z^{stretching} = \int_{-t(1-\nu\varepsilon_z)/2}^{t(1-\nu\varepsilon_z)/2} \sigma_x H(1+\varepsilon_z) y dy = \frac{\pi EHt^3\,(\varepsilon_z+1)\,(1-\nu\varepsilon_z)^3}{6nL\,(1-\nu^2)}. \quad \text{[S13]}$$

In Fig. S13*C* we compare analytical (Eqs. S11 and S13) and FE results (using Eqs. S7 and Eqs. S4 with Eq. S8 and Eq. S9) for $n = 4$ and 8. We find a great agreement between the two sets of data, confirming the validity of our numerical analysis.

***Curved kirigami sheets..*** To investigate the effect of the residual stresses generated during rolling on the mechanical response of our kirigami cylinders, we also performed simulations on initially curved ( stress-free) models. The curved models are created in SolidWorks (Version 2016) by wrapping a flat cell around a curved sector of a cylindrical surface with radius $r = Ln/(2\pi)$. To stretch them axially, we then apply the following periodic boundary conditions to their *left* and the *right* edges:

$$
\begin{aligned}
&u_\rho^{R_i} = u_\rho^{L_i},\\
&u_\phi^{R_i} = u_\phi^{L_i},\\
&u_z^{R_i} = u_z^{L_i},\\
&\theta_\rho^{L_i} = \theta_\rho^{R_i} = 0,\\
&\theta_\phi^{L_i} = \theta_\phi^{R_i},\\
&\theta_z^{L_i} = \theta_z^{R_i} = 0, \quad i = 1, 2, ...N.
\end{aligned} \tag{S14}
$$

As for the *top* and *bottom* edges, we apply the same periodic boundary used for the case of the rolled kirigami sheets.

Additional numerical results are provided in Figs. S14-S21.

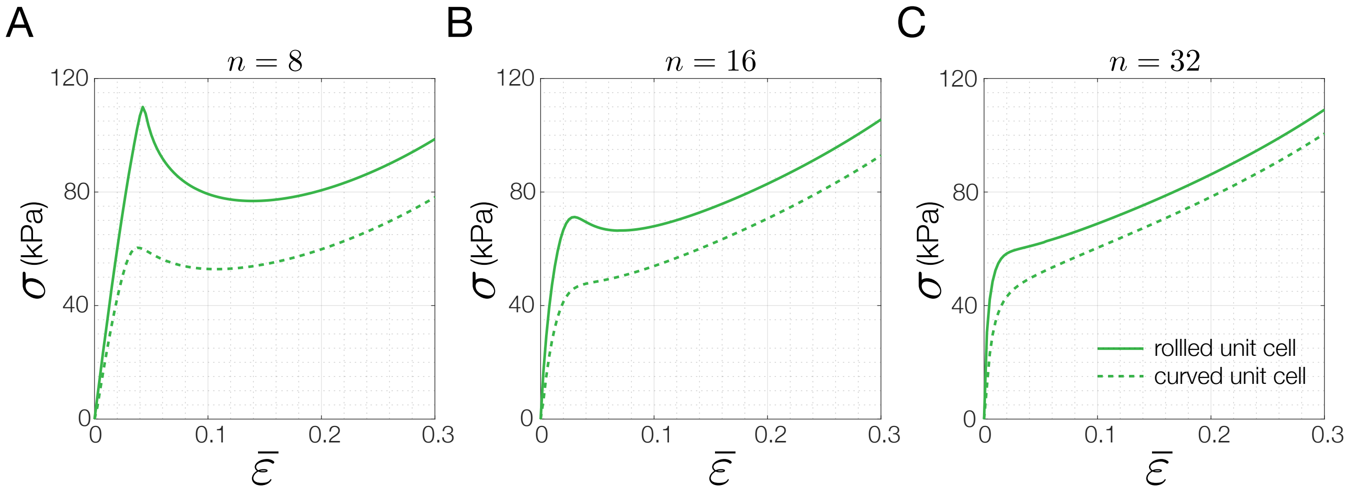


**Fig. S14.** Comparison between the stress-strain curve of curved and rolled unit kirigami sheets with triangular cuts. We consider unit cells with $l = 12$mm and $\delta = 0.75$mm and use (*A*) $n = 8$, (*B*) $n = 16$ and (*C*) $n = 32$. We observe that for small $n$ (i.e. large curvature) the rolled kirigami sheets are significantly stiffer than the initially curved ones. However, as the number of units along the circumference increases their responses converge to each other. Also, we find that for the rolled kirigami sheets the overshoot in stress-strain curve is more pronounced than for initially curved ones.

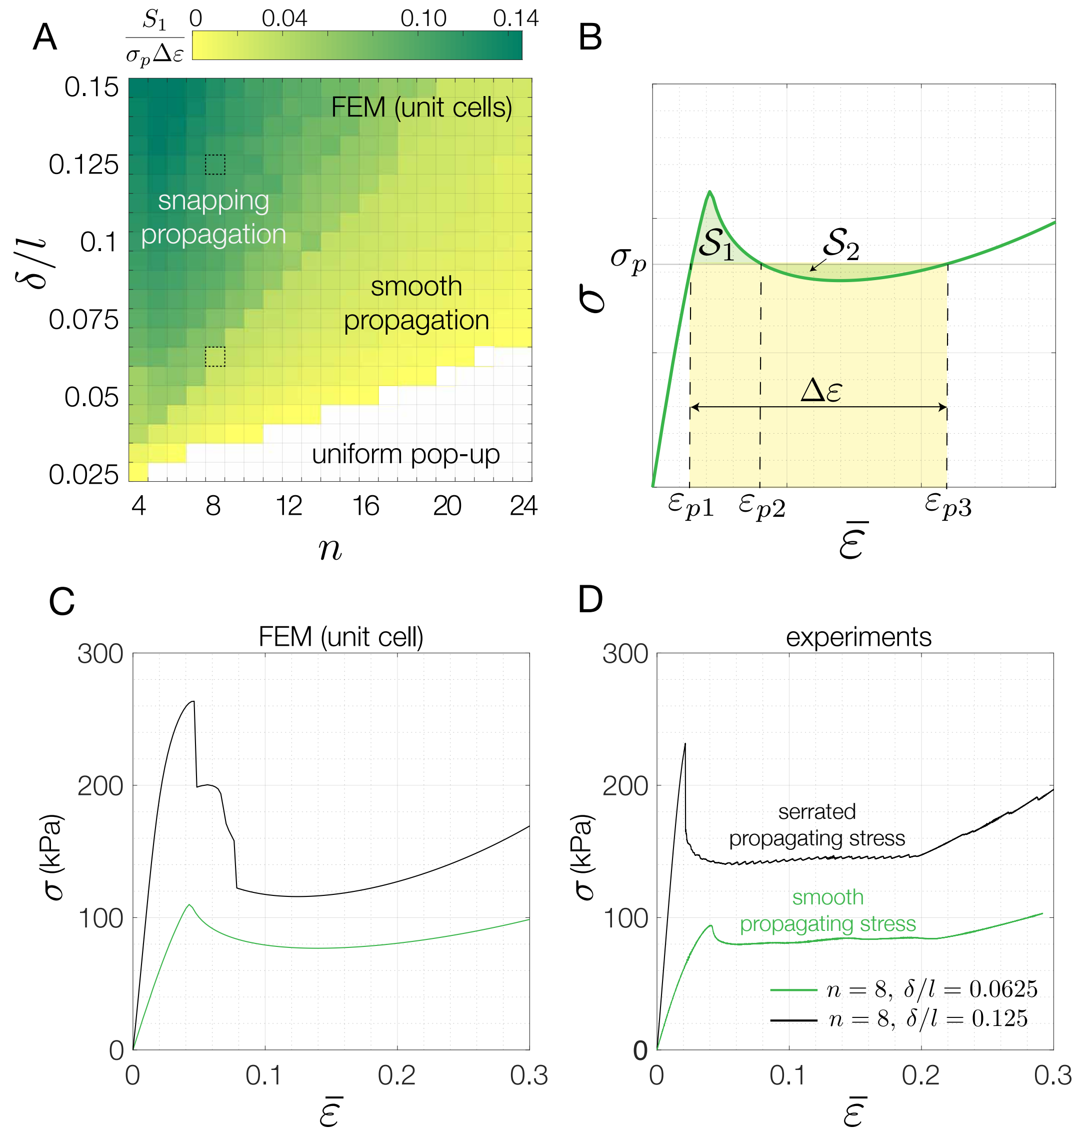


**Fig. S15.** (*A*) Phase diagram for kirigami shells with triangular cut pattern. The color indicates the energy barrier $\mathcal{S}_1$ (see shaded green area in *B*) normalized by the total energy required for phase transition (i.e. $\sigma_p\Delta\varepsilon$). The white region represents uniform pop-up. This plot is obtained by simulating the response of 441 rolled unit cells. The type of behavior is determined based on the obtained stress-strain curve. If the stress monotonically increases as a function of the strain, a uniform pop-up is triggered; otherwise a propagative instability. (*B*) Schematic strain-stress curve of a unit cell of a kirigami shell indicating the energy barrier $\mathcal{S}_1$, propagation stress $\sigma_p$ obtained by the condition $\mathcal{S}_1 = \mathcal{S}_2$, strain increment required for phase transition $\Delta\varepsilon$, two stable strains at unpopped ($\varepsilon_{p1}$) and popped ($\varepsilon_{p3} = \varepsilon_{p1} + \Delta\varepsilon$) states and the intermediate unstable strain $\varepsilon_{p2}$. (*C*) FE stress-strain curves obtained by simulating two rolled unit cells ($n = 8$, $L = 12$ mm) with triangular cuts indicated in phase diagram (*A*) with dashed squares and characterized by FE $\delta/l = 0.0625$ and $\delta/l = 0.125$. (*D*) Experimental stress-strain curves for two kirigami shells built using the unit cells considered in C. Note that the sharp drop in load found in the stress-strain curve of the unit cell with $\delta/l = 0.125$ results in a discrete sequence of small drops during propagation of pop-ups in the finite-sized structure, each corresponding to the opening of one row of cuts. For such snapping propagation regime we expect a fraction of energy to be dissipated, so that the use of Maxwell's rule (which is based on the assumption of a conservative system) is not rigorous.

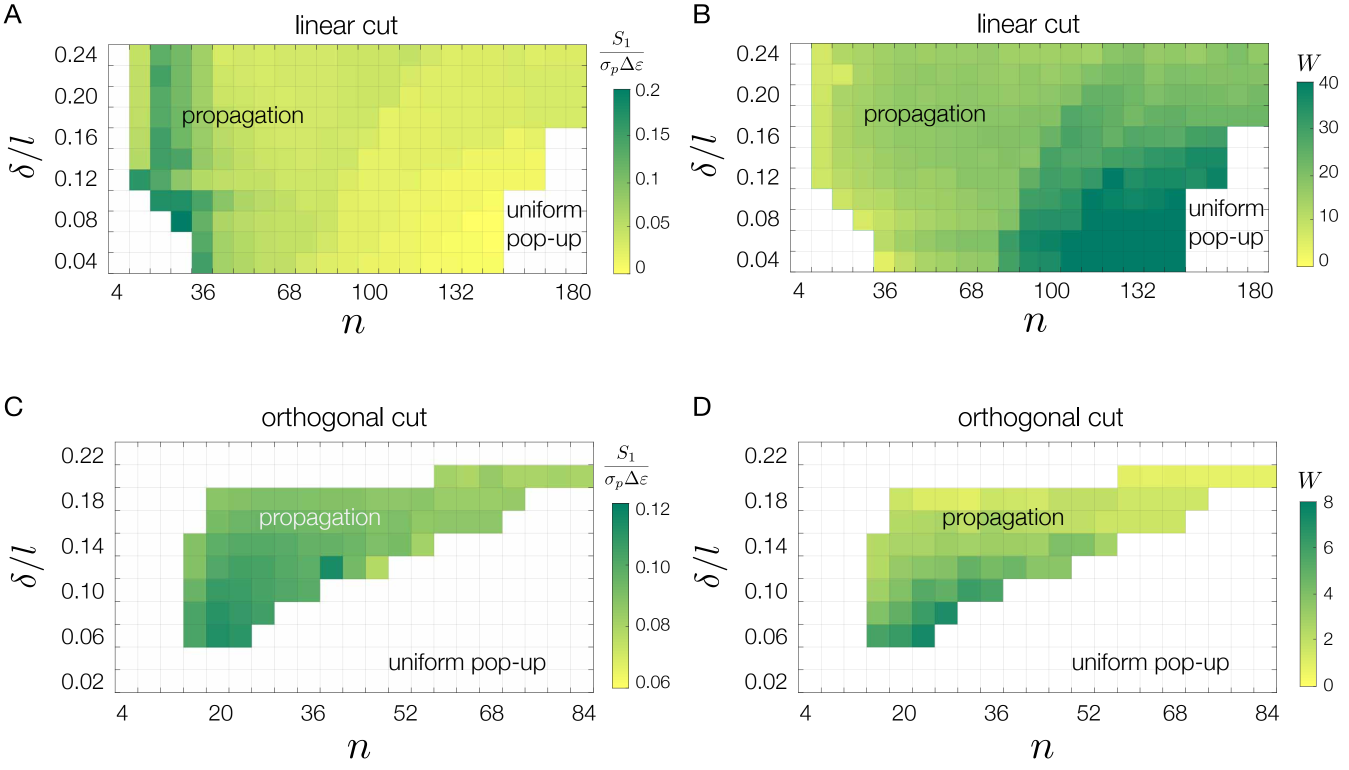


**Fig. S16.** Phase diagrams for kirigami shells with (*A*, *B*) linear and (*C*, *D*) orthogonal cut patterns obtained by simulating respectively 253 and 231 rolled unit cells. The color in *A* and *C* indicates the energy barrier $\mathcal{S}_1$ (see shaded green area in Fig. S15*B*) normalized by the total energy required for phase transition (i.e. $\sigma_p\Delta\varepsilon$) while in *B* and *D*, the color shows $W$ the width of the transition zone in the unit of number of units. The white region represents uniform pop-up. These plots are obtained as described in the caption of Fig. S15. Note that, since the response of the linear pattern is very sensitive to imperfection, the phase diagram shown in (*A*) is obtained by imposing an initial imperfection with magnitude equal to $0.1t$. Moreover, since for most configurations the energy barrier is very small, we expect only a limited number of them (characterized by large $\mathcal{S}_1$) to exhibit a well visible propagation of pop-ups.

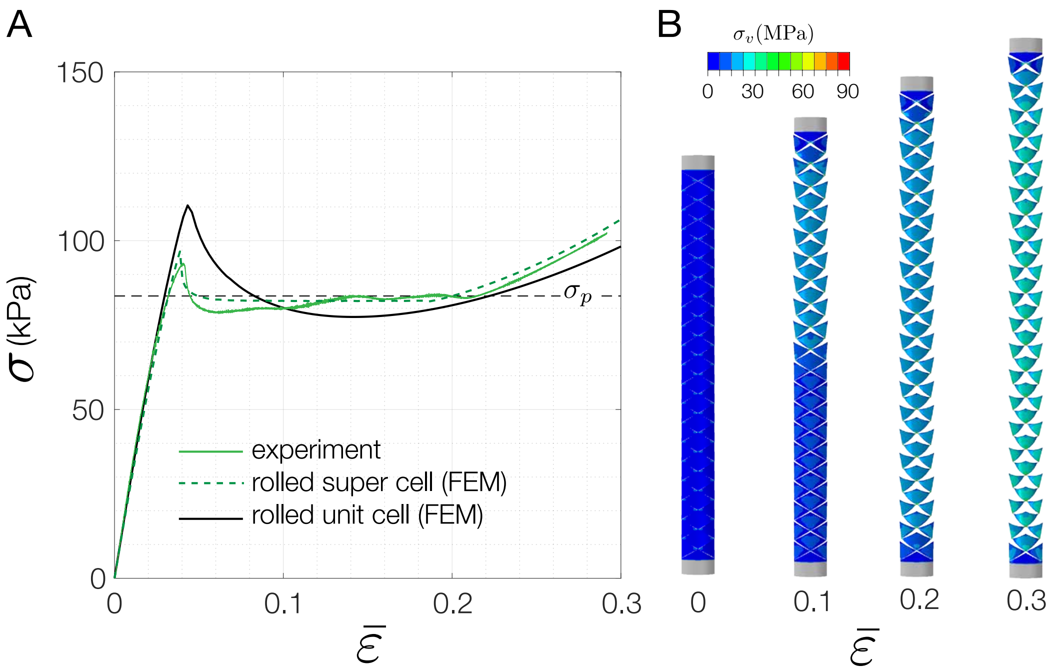


**Fig. S17.** (*A*) Stress-strain response for a kirigami shell with triangular pattern characterized by $l = 12$ mm and $\delta = 0.75$ mm. Results from FE simulations conducted on a rolled $20 \times 1$ super-cell are compared to experiments and to the numerical predictions obtained for the corresponding unit cell. Excellent agreement between experiments and FE simulations is found. (*B*) Snapshots of the deformed super-cell at different applied strain $\bar{\varepsilon}$. In the snapshots we also show the *von Mises* stress distributions.

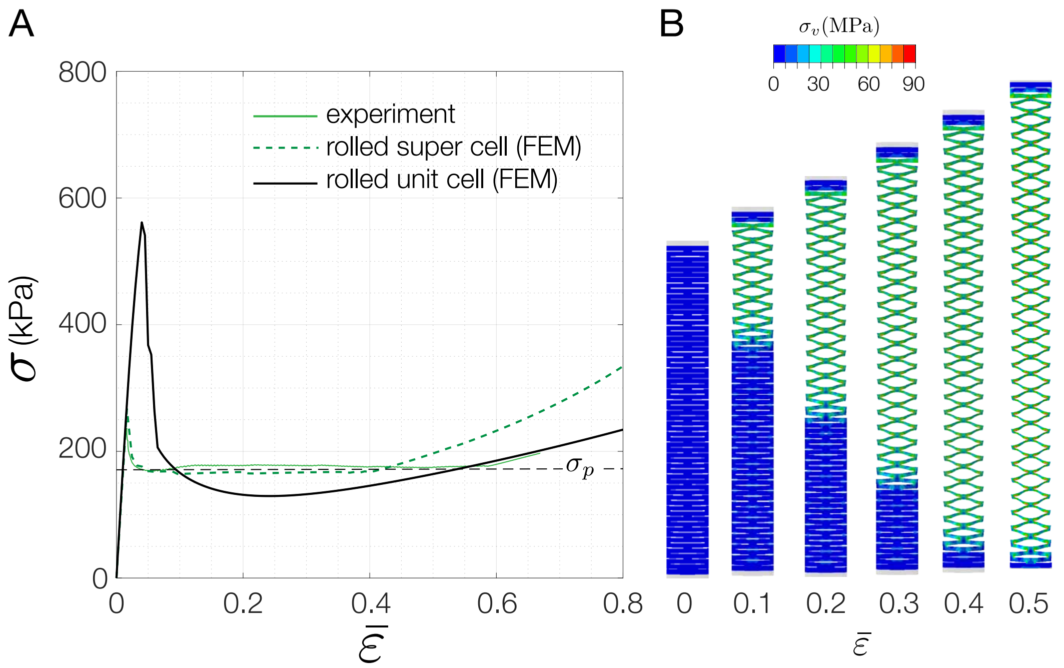


**Fig. S18.** (*A*) Stress-strain response for a kirigami shell with linear pattern characterized by $l = 12$ mm and $\delta/l = 0.2$. Results from FE simulations conducted on a rolled $20 \times 1$ super-cell are compared to experiments and to the numerical predictions obtained for the corresponding unit cell. Excellent agreement between experiments and FE simulations is found. (*B*) Snapshots of the deformed super-cell at different applied strain $\bar{\varepsilon}$. In the snapshots we also show the *von Mises* stress distributions.

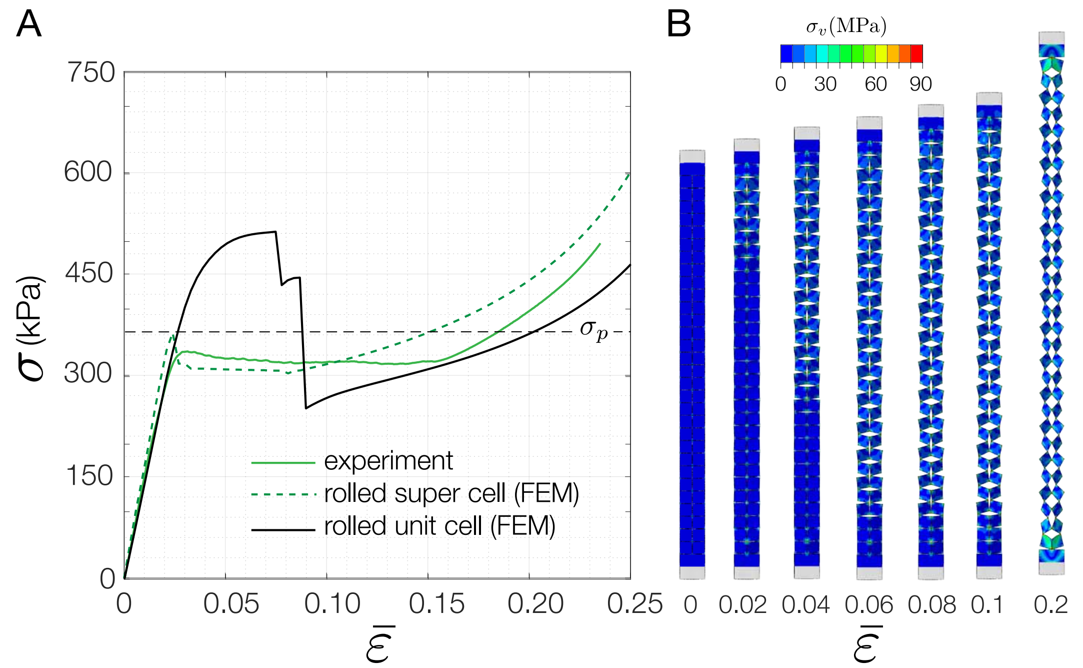


**Fig. S19.** (*A*) Stress-strain response for a kirigami shell with orthogonal pattern characterized by $l = 6$ mm and $\delta/l = 0.08$. Results from FE simulations conducted on a rolled $20 \times 1$ super-cell are compared to experiments and to the numerical predictions obtained for the corresponding unit cell. Excellent agreement between experiments and FE simulations is found. (*B*) Snapshots of the deformed super-cell at different applied strain $\bar{\varepsilon}$. In the snapshots we also show the *von Mises* stress distributions.

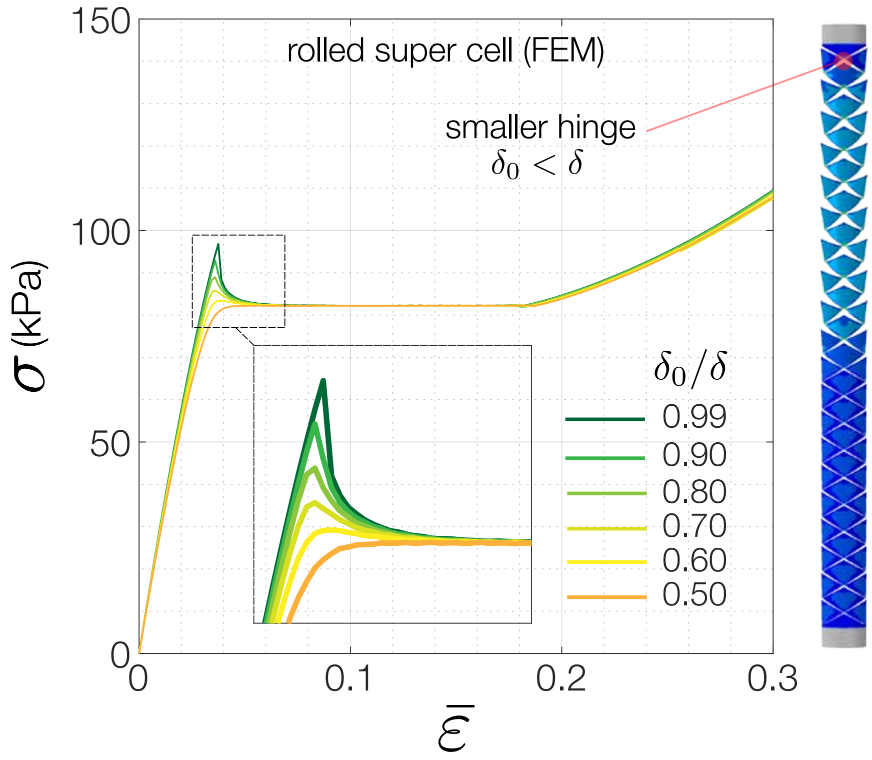


**Fig. S20.** The effect of the imperfection size on the stress-strain behavior of kirigami shell is investigated by conducting FEM simulations on super-cells with a triangular cut pattern characterized by $\delta/l = 0.0625$, $l = 12$mm and $n = 8$. In our models the size of the hinge in the top unit cell is reduced to $\delta_0 < \delta$. We find that as $\delta_0/\delta$ increases the overshoot in the stress-strain curve decreases and eventually vanishes for $\delta_0/\delta$=0.5. By contrast, the propagation stress $\sigma_p$ is not affected by $\delta_0/\delta$.

**B. Theoretical model.** Both our experiments and our FE simulations show that in thin cylindrical kirigami shells subjected to tensile loading the buckling induced pop-up process initially localizes near an imperfection and then, as the deformation is increased, progressively spreads through the cylinder at constant stress. Moreover, our FE simulations indicate that the stress-strain response of a rolled kirigami unit cell is non-monotonic, characterized by a peak, a subsequent drop in load and final stiffening (see Fig. 3B of the main text). Guided by these observations, here we develop models to characterize the behavior of our kirigami structures.

***Maxwell construction.*** Maxwell construction (10) applied to the stress-strain response of a unit cell enables us to identify several key parameters that characterize the behavior of our curved kirigami shell. Specifically, by equating the area of the two lobes formed by the $\sigma(\varepsilon)$ curve (i.e. by imposing $\mathcal{S}_1 = \mathcal{S}_2$) we can identify $(i)$ the propagation stress $\sigma_p$, $(ii)$ the energy barrier $\mathcal{S}_1$ and $(iii)$ the critical strains $\varepsilon_{p1}$, $\varepsilon_{p2}$ and $\varepsilon_{p3}$ (see Fig. S21). While for $\bar{\varepsilon} < \varepsilon_{p1}$ the structure deforms homogeneously and all triangular features are unpopped, for $\varepsilon_{p1} < \bar{\varepsilon} < \varepsilon_{p3}$ the pop-up process initiated at the top end of the sample spreads towards the other end. However, it is important to note that Maxwell construction does not provides any information on the width and the shape of the transition zone. This motivates the derivation of the more detailed and comprehensive model described below.

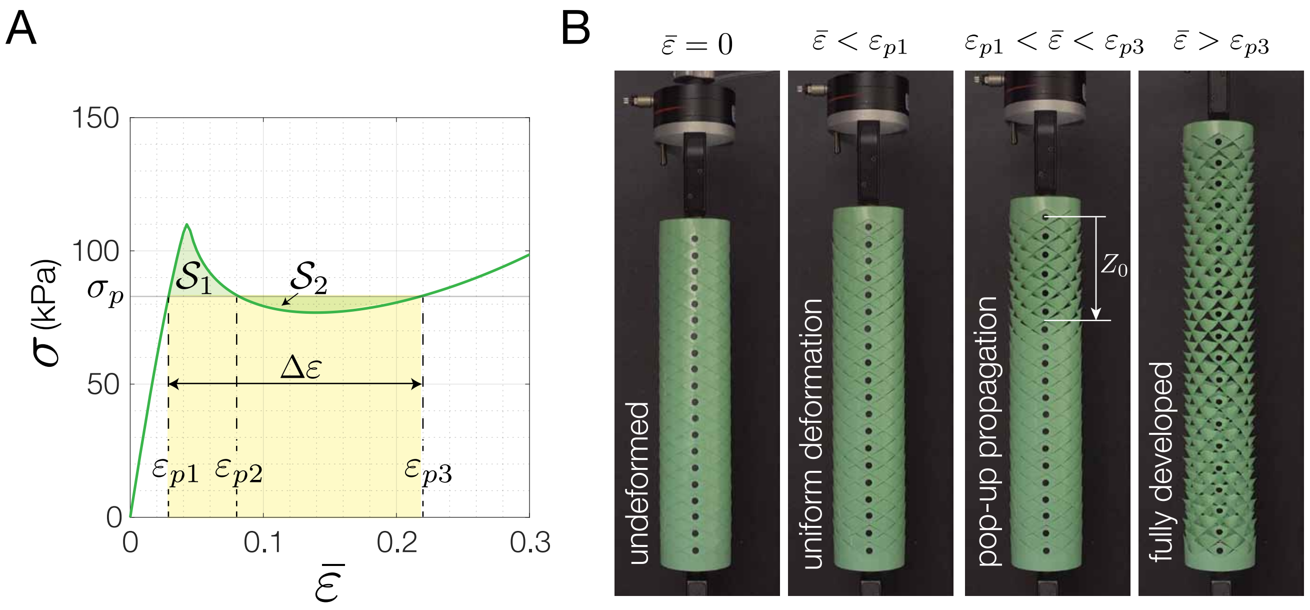


**Fig. S21.** (*A*) Typical stress-strain curve for a rolled kirigami unit cell. Several parameters can be identified from Maxwell construction (i.e. by imposing $\mathcal{S}_1 = \mathcal{S}_2$). (*B*) Experimental images of a kirigami shell fabricated by rolling a sheet with a triangular pattern characterized by $\delta/l$ = 0.0625 (with by $l$ = 12 mm and $n$ = 8 unit cells along the circumference) at $\bar{\varepsilon} = 0$ (before the test starts), $\bar{\varepsilon} < \varepsilon_{p1}$ (before the pop-up process starts), $\varepsilon_{p1} < \bar{\varepsilon} < \varepsilon_{p3}$ (during propagation of pop-ups) and $\bar{\varepsilon} > \varepsilon_{p3}$ (after all triangular features popped-up).

***Detailed model.*** To predict the strain distribution during the propagation of the pop-ups, we use a 1D array of non-linear springs (see Fig. S22). In our model the response of the $i$-th spring is described by

$$F_i(u_i,\, u_{i+1}) = nLt \times \sigma\left(\varepsilon_i\right), \quad \text{with } \varepsilon_i = \frac{u_{i+1} - u_i}{H}, \qquad \text{[S15]}$$

where $\sigma(\varepsilon_i)$ is the non-linear stress-strain response of the unit cell and $u_i$ and $u_{i+1}$ denote the axial displacement at the two ends of the spring.

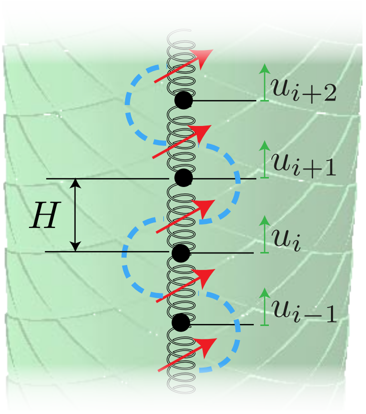


**Fig. S22.** The response of our kirigami structures is captured using a 1D array of non-linear springs connected in series. To accurately capture the effect of strain gradient we introduce an additional term (represented by the blue dashed lines in the schematic) that connects the response of the $i$-th spring to that of the two neighboring ones.

It follows that for a system comprising a $N$ springs the total strain energy is given by

$$U = \sum_{i=1}^{N} \int_0^{u_{i+1}-u_i} F_i \mathrm{d}(u_{i+1} - u_i) = \sum_{i=1}^{N} nLt \int_0^{u_{i+1}-u_i} \sigma \left( \frac{u_{i+1} - u_i}{H} \right) \mathrm{d}(u_{i+1} - u_i), \qquad \text{[S16]}$$

from which the equilibrium equation can be derived as

$$\frac{\partial U}{\partial u_i} = 0, \quad \text{for } i = 1, ..., N. \qquad \text{[S17]}$$

To test the ability of our discrete model to capture the response of our kirigami structures, we focus on a kirigami shell with $n = 8$ and triangular cuts characterized by $\delta/l = 0.0625$. We first use FE analyses to determine the stress-strain behavior of the unit cell (see Fig. S23*A*). Then, we use both FE analyses and our discrete model based on Eq. S16 to investigate the response of a cylindrical shell comprising two rows of unit cells (i.e. $N = 2$) when subjected to two different loading conditions, case #1 and case #2 (see Fig. S23*B*). For case #1, we stretch the two unit cells homogeneously (i.e. we impose $\varepsilon_1 = \varepsilon_2$ and progressively increase $\varepsilon_1$), whereas for Case #2 we stretch the first unit cell, while keeping the second one closed (i.e. we set $\varepsilon_2 = 0$ and progressively increase $\varepsilon_1$), inducing a highly inhomogeneous deformation. As it can be seen in Figs. S23*C* and *D*, the inhomogeneous deformation (i.e. the strain gradient) of case #2 makes the structure significantly stiffer - a feature that cannot be captured by our simple model.

To properly account for the effect of the strain gradient, which significantly affects the response of our system given the strong coupling between its unit cells, we modify the strain energy given in Eq. S16 to

$$U = \sum_{i=1}^{N} nLt \int_0^{u_{i+1}-u_i} \sigma \left( \frac{u_{i+1} - u_i}{H} \right) \mathrm{d}(u_{i+1} - u_i) + \sum_{i=2}^{N} \frac{1}{2} nLtG \left( u_{i+1} - 2u_i + u_{i-1} \right)^2. \qquad \text{[S18]}$$

where the last term is introduced to capture the effect of the strain gradient (8, 9) (see Fig. S22*B*). Note that the coefficient $G$ in Eq. S18 can be easily determined using the two FE simulations shown

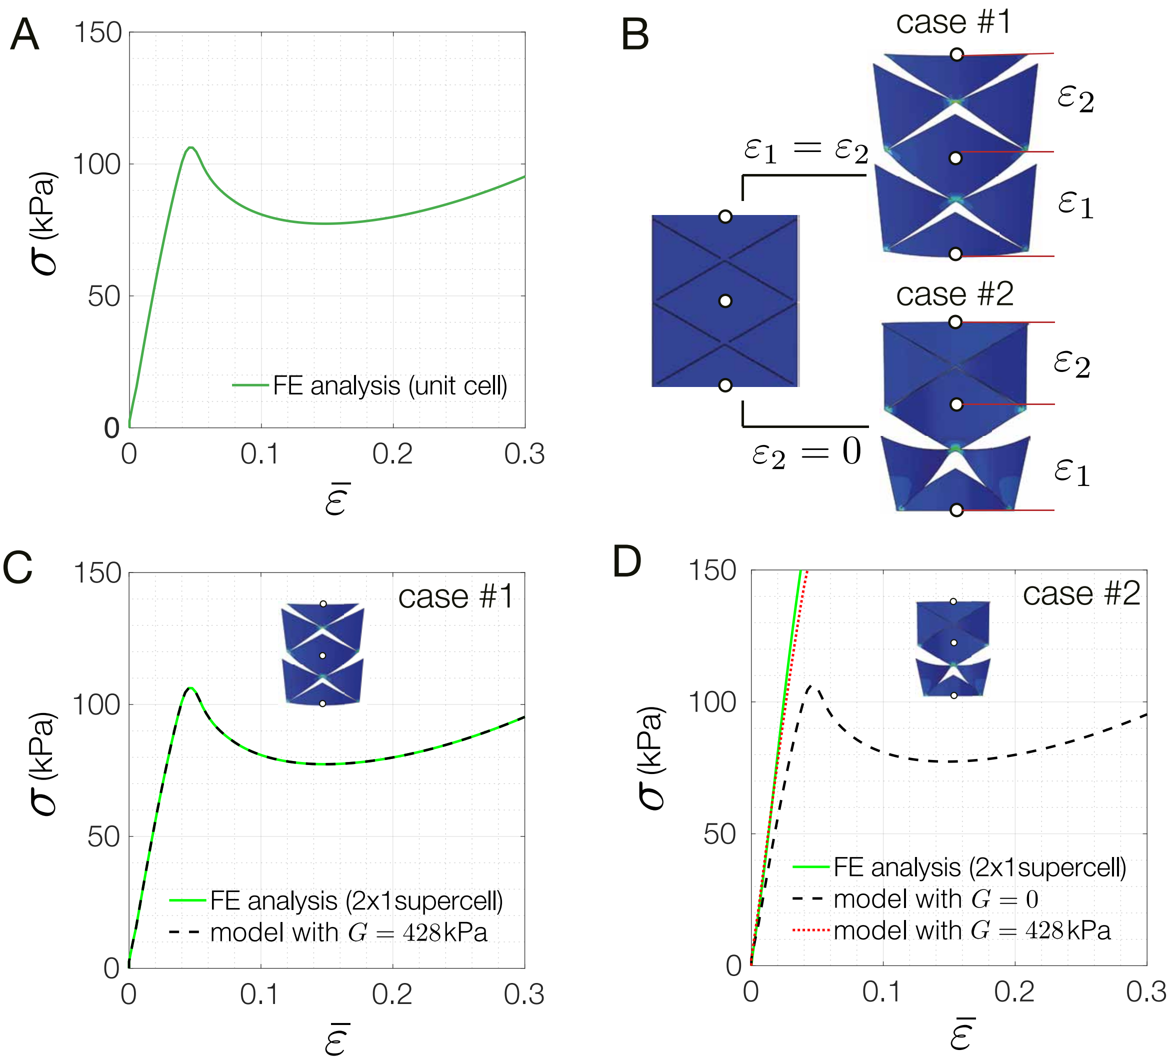


**Fig. S23.** (*A*) Stress-strain curve for a unit cell of a kirigami shell with $n$=8 and $\delta/l = 0.0625$ as predicted by our FE analysis. (*B*) We simulate the response of a super-cell comprising $2 \times 1$ unit cells when: (case $\#1$) the two unit cells are stretched homogeneously (i.e. we impose $\varepsilon_1 = \varepsilon_2$ and progressively increase $\varepsilon_1$) and (case $\#2$) the first unit cell is stretched while the second one is kept closed (i.e. we set $\varepsilon_2 = 0$ and progressively increase $\varepsilon_1$). (*C*) The response of the structure for case $\#1$ obtained via FE analysis is nicely captured by both the model with $G = 0$ and $G = 428$ kPa. (*D*) The response of the structure for case $\#1$ obtained via FE analysis is not captured by the model with $G = 0$, whereas is nicely captured by the model with $G = 428$ kPa, motivating the introduction of the strain gradient term.

in Fig. S23. More specifically, since the initial stiffness $K$ predicted using Eq. S18 for Case $\#1$ and Case $\#2$ is given by

$$\begin{aligned} K_{Case\,\#1} &= \left.\frac{\partial^2 U_{Case\,\#1}}{\partial(u_2-u_1)^2}\right|_{u_1=u_2=0} = \frac{nLt}{H}\left.\frac{\partial\sigma(\varepsilon)}{\partial\varepsilon}\right|_{\varepsilon=0}, \\ K_{Case\,\#2} &= \left.\frac{\partial^2 U_{Case\,\#2}}{\partial(u_2-u_1)^2}\right|_{u_1=u_2=0} = \frac{nLt}{H}\left.\frac{\partial\sigma(\varepsilon)}{\partial\varepsilon}\right|_{\varepsilon=0} + nLtG, \end{aligned} \quad [S19]$$

it follows that

$$G = \frac{K_{Case\,\#2} - K_{Case\,\#1}}{nLt}. \quad [S20]$$

In Figs. S23$C$ and $D$ we compare the results of our discrete model based on Eq. S18 with those

obtained via FE analyses. We find that using $G = 428\,\text{kPa}$ (value determined using Eq. S20) the model captures very well the response of the structure for both loading cases, indicating that the coupling constant $G$ should be included in the model to correctly capture the response of our system. On the other hand, it is interesting to note that if a structure consists of units that are not strongly coupled so that $K_{Case\,\#1} - K_{Case\,\#2} \to 0$, then $G \to 0$ and the term introduced to capture the effect of strain gradient vanishes.

Having established a simple discrete model capable of capturing the non-linear response of our kirigami structures, we now use it to investigate the characteristics of the triggered propagative instability. To this end, since our experiments indicate that the propagation of the instability-induced pop-up process occurs at a constant axial stress $\sigma_p$, we write the total potential energy of the system as,

$$\begin{aligned}\Pi =& U - F_p(u_{N+1} - u_1)\\ =& \sum_{i=1}^{N} nLt \int_0^{u_{i+1}-u_i} \sigma\left(\frac{u_{i+1}-u_i}{H}\right) \mathrm{d}(u_{i+1}-u_i) + \sum_{i=2}^{N} \frac{1}{2} nLtG\left(u_{i+1} - 2u_i + u_{i-1}\right)^2 - F_p(u_{N+1} - u_1),\end{aligned} \quad [S21]$$

with

$$F_p = nLt\sigma_p. \quad [S22]$$

We then derive the equilibrium equations by imposing

$$\frac{\partial \Pi}{\partial u_i} = 0, \quad \text{for } i = 1, ..., N. \quad [S23]$$

and obtain

$$\begin{aligned}&\sigma\left(\frac{u_{i+1}-u_i}{H}\right) - \sigma\left(\frac{u_i - u_{i-1}}{H}\right)\\ &\qquad - G\left[u_{i+2} - 4u_{i+1} + 6u_i - 4u_{i-1} + u_{i-2}\right] = 0, \quad \text{for } = 3, \; ..., \; N-1\end{aligned} \quad [S24]$$

which can be rewritten in terms of the local strain $\varepsilon_i = (u_{i+1} - u_i)/H$ as

$$\mathcal{E}_i = \sigma\left(\varepsilon_i\right) - \sigma\left(\varepsilon_{i-1}\right) - G\left(\varepsilon_{i+1} - 3\varepsilon_i + 3\varepsilon_{i-1} - \varepsilon_{i-2}\right) = 0, \quad \text{for } = 3, \; ..., \; N-1 \quad [S25]$$

Next, we introduce a continuous function $\varepsilon(Z)$, which interpolates the discrete variable $\varepsilon_i$ as

$$\varepsilon(Z = i\,H) = \varepsilon_i, \quad [S26]$$

where $Z$ denotes the position along the structure. Using Taylor expansion, the strains $\varepsilon_{i\pm1}$ and $\varepsilon_{i\pm2}$ can then be expressed as

$$\varepsilon_{i+p} = \varepsilon(iH) + pH\frac{\mathrm{d}\varepsilon(iH)}{\mathrm{d}Z} + \frac{p^2H^2}{2}\frac{\mathrm{d}^2\varepsilon(iH)}{\mathrm{d}Z^2} + \frac{p^3H^3}{6}\frac{\mathrm{d}^3\varepsilon(iH)}{\mathrm{d}Z^3} + \mathbf{O}\left(\frac{\mathrm{d}^4\varepsilon(iH)}{\mathrm{d}Z^4}\right), \quad [S27]$$

with $p$ =-2, -1, 1 and 2. By substituting Eqs. S27 into

$$\mathcal{E}_{i+1} + \mathcal{E}_i = \sigma\left(\varepsilon_i\right) - \sigma\left(\varepsilon_{i-1}\right) - G\left(\varepsilon_{i+2} - 2\varepsilon_{i+1} + 2\varepsilon_{i-1} - \varepsilon_{i-2}\right) = 0 \quad [S28]$$

and retaining terms up to the third order, we obtain

$$GH^2\frac{\mathrm{d}^3\varepsilon}{\mathrm{d}Z^3} - \frac{\mathrm{d}\sigma(\varepsilon)}{\mathrm{d}Z} = 0, \quad [S29]$$

which we integrate with respect to $Z$ to get

$$GH^2 \frac{\mathrm{d}^2\varepsilon}{\mathrm{d}Z^2} - \sigma(\varepsilon) + C_1 = 0, \tag{S30}$$

where $C_1$ is an integration constant. If we assume that at $Z \to -\infty$ the structure is unpopped (so that $\mathrm{d}^2\varepsilon/\mathrm{d}Z^2|_{-\infty} = 0$) and define $\varepsilon_{p1}$ as the strain experienced by the unpopped unit cells when subjected to a constant stress $\sigma_p$ (i.e. $\varepsilon(Z \to -\infty) = \varepsilon_{p1}$, where $\varepsilon_{p1}$ is the smallest root of $\sigma(\varepsilon) - \sigma_p = 0$), we find that

$$C_1 = \sigma(\varepsilon_{p1}) = \sigma_p. \tag{S31}$$

Substitution of Eq. S31 into Eq. S30 yields

$$GH^2 \frac{\mathrm{d}^2\varepsilon}{\mathrm{d}Z^2} = \sigma(\varepsilon) - \sigma_p, \tag{S32}$$

which can be solved to obtain the spatial profile of the strain, $\varepsilon(Z)$, for a given $\sigma_p$.

Next, to gain more insight into the response of our kirigami structures, we multiply Eq. S32 by $d\varepsilon/dZ$ and integrate with respect to $Z$ to get

$$\frac{1}{2} GH^2 \left( \frac{\mathrm{d}^2\varepsilon}{\mathrm{d}Z^2} \right)^2 = -\int_0^{\varepsilon} \left[ \sigma(\varepsilon') + \sigma_p \right] \mathrm{d}\varepsilon' \tag{S33}$$

which can be viewed as the sum of the kinetic energy (with respect to the pseudo-time $Z$) and the potential energy of a fictitious particle of mass $GH^2$ (13). Thus, the solution $\varepsilon(Z)$ of Eq. S32 describes the motion of such particle in the potential

$$V_{eff}(\varepsilon) = -\int_0^{\varepsilon} \left[ \sigma(\varepsilon') - \sigma_p \right] \mathrm{d}\varepsilon'. \tag{S34}$$

Specifically, the existence of propagation of pop-ups requires a $V_{eff}$ with two stable configurations (located at $\varepsilon_{p1}$ and $\varepsilon_{p3}$) characterized by the same energy level. Under these conditions, a fictitious particle leaving the first peak at rest can reach the second one with a vanishing "velocity" $d\varepsilon/dZ$ and this corresponds to a transition that brings each unit cell from $\varepsilon_{p1}$ and $\varepsilon_{p3}$. Focusing on the kirigami unit cells investigated in this study, we find that, if the stress-strain curve of the unit cell is monotonic (as for our flat unit cells - see Fig. S24*A*), $V_{eff}$ has a single stable configuration (see Fig. S24*B*) and propagation of pop-ups cannot exist. By contrast, if the stress-strain curve is non-monotonic (and characterized by an up-down-up behavior - see Fig. S24*C*) and $\sigma_p$ is chosen so that the equation $\sigma(\varepsilon) - \sigma_p = 0$ has three real roots, $V_{eff}$ has two stable configurations (see Fig. S24*C*) located at $\varepsilon_{p1}$ and $\varepsilon_{p3}$ (see Fig. S24*D*). However, these two configurations are characterized by the same energy only when $\sigma_p$ corresponds to the Maxwell stress (i.e. the stress for which $\mathcal{S}_1 = \mathcal{S}_2$) - an observation that confirms the validity of or model. Inspection of Eq. S33 also provides insights on the width of the transition zone. More specifically, since the motion of the fictitious particles gets slower as its mass $GH^2$ increases, we expect the transition zone to becomes wider for larger $GH^2$ (i.e. for structures characterized by a larger coupling constant $G$). Therefore, given a specific non-monotonic stress strain curve of the unit cell $\sigma(\varepsilon)$, Eq. S32 can be numerically solved to obtain the strain distribution within the structure during the propagation of the pop-ups.

Finally, we validate the ability of our model to capture the response of our kirigami structures by comparing the evolution of the strain along the cylindrical kirigami shells as predicted by our model and measured in experiments at different level of applied strain for shells with triangular pattern

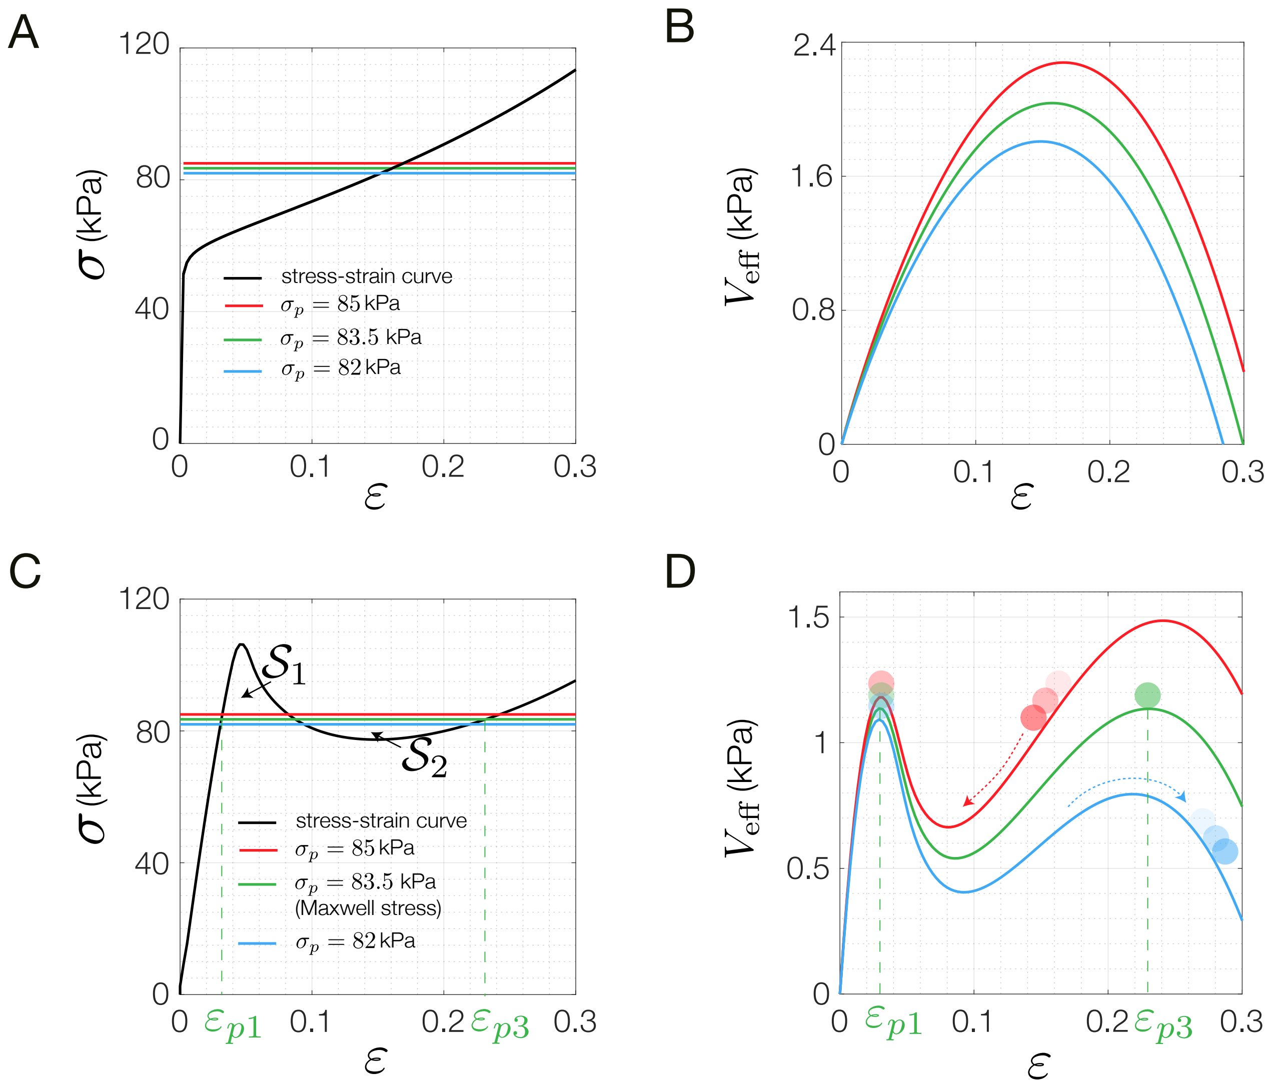


**Fig. S24.** (*A*) Stress-strain curve of a flat unit cell with triangular cuts characterized by $\delta/l = 0.0625$ as obtained via FE analysis. (*B*) Corresponding potential energy $V_{\text{eff}}$ as a function of applied strain $\varepsilon$ for three different $\sigma_p$ (note that the color of the curves corresponds to the $\sigma_p$ indicated in A). (*C*) Stress-strain curve of a rolled unit cell with $n$=8 and triangular cuts characterized by $\delta/l = 0.0625$ as obtained via FE analysis. (*D*) Corresponding potential energy $V_{\text{eff}}$ as a function of applied strain $\varepsilon$ for three different $\sigma_p$ (note that the color of the curves corresponds to the $\sigma_p$ indicated in *A*)

(with $\delta/l = 0.0625$ and $n = 8$ - Fig. S25*A*), linear pattern (with $\delta/l = 0.2$ and $n = 20$ - Fig. S25*B*) and orthogonal pattern (with $\delta/l = 0.08$ and $n = 20$ - Fig. S25*C*). Note that the model predictions are obtained by numerically integrating Eq. S32 with $\sigma(\varepsilon)$ predicted by our FE simulations on the unit cell and $\sigma_p$ equal to the Maxwell stress. Moreover, since the solution of Eq. S32 is translational invariant with respect to $Z$, the position of the propagation front $Z_0$ (see Fig. S21*B*) for a given applied strain $\bar{\varepsilon}$ can be determined from the compatibility condition

$$\bar{\varepsilon} = \frac{1}{Z_q - Z_p} \int_{Z_p}^{Z_q} \varepsilon(Z - Z_0)\, \mathrm{d}Z. \qquad \text{[S35]}$$

where, to minimize boundary effects, we choose $(p,\, q) = (3,\, 18)$, $(5,\, 55)$ and $(1,\, 30)$ for structures with triangular, linear and orthogonal patterns, respectively. In Fig. S25 we find a very nice agreement between the experimental results and the predictions of our model, with our model

correctly predicting the very different widths and amplitudes of the transition zones for the three structures as well as their position as a function of the applied deformation.

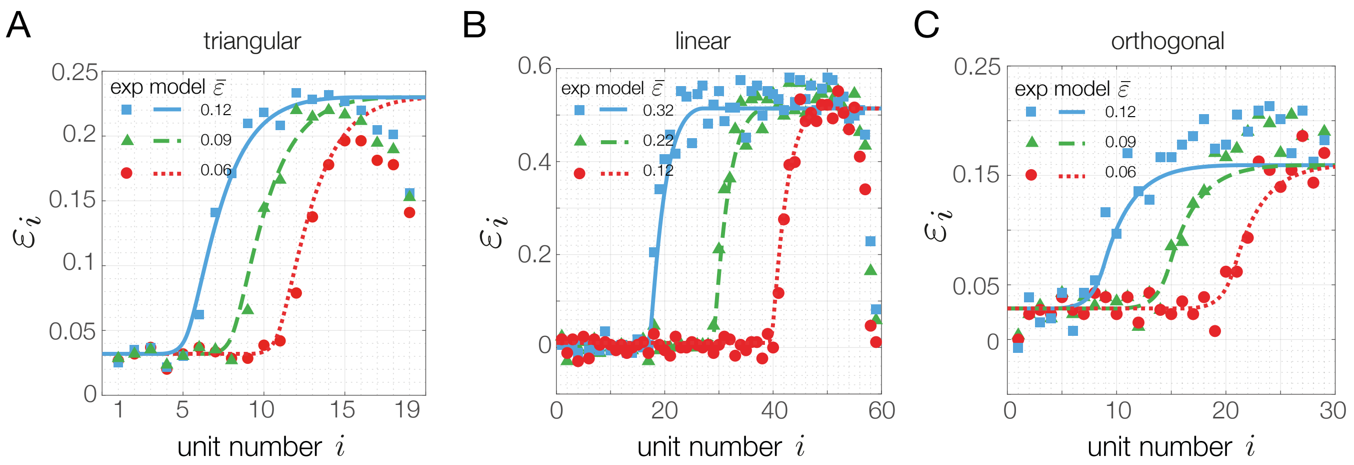


**Fig. S25.** Comparison between the evolution of the strain along the cylindrical kirigami shells as measured in experiments and obtained by numerically integrating Eq. S32 for (a) a triangular pattern with $\delta/l = 0.0625$ and $n = 8$, (b) a linear pattern with $\delta/l = 0.2$ and $n = 20$ and (c) an orthogonal pattern with $\delta/l = 0.08$ and $n = 20$.

Special case with analytical solution. While Eq. S36 is nonlinear, it is interesting to note that it admits analytical solution if the stress-strain curve of a unit cell is described by a third order polynomial,

$$\sigma(\varepsilon) = B_1\varepsilon + B_2\varepsilon^2 + B_3\varepsilon^3. \quad \text{[S36]}$$

Substitution of Eq. S36 into the continuum governing equation Eq. S32 yields,

$$\frac{\mathrm{d}^2\varepsilon}{\mathrm{d}Z^2} = \frac{B_1\varepsilon + B_2\varepsilon^2 + B_3\varepsilon^3 - \sigma_p}{GH^2}, \quad \text{[S37]}$$

which is a Klein-Gordon equation with quadratic and cubic nonlinearities (12). Such equation yields analytical solution of the form

$$\varepsilon(Z) = \varepsilon_{p1} + \frac{\Delta\varepsilon}{2}\left[1 + \tanh\left(\frac{Z - Z_0}{W}\right)\right], \quad \text{[S38]}$$

where $\varepsilon_{p1}$ and $\varepsilon_{p1} + \Delta\varepsilon$ denote the strain experienced by the unit cells in the closed/unpopped and open/popped configuration, respectively, $W$ is the width of the transition zone and $Z_0$ provides the position of such transition zone. By substituting the solution S38 into Eq. S32 we find that the latter is identically satisfied only if

$$\Delta\varepsilon = \frac{2\sqrt{B_2^2 - 3B_1B_3}}{\sqrt{3}B_3}, \quad \varepsilon_{p1} = -\frac{\Delta\varepsilon}{2} - \frac{B_2}{3B_3}, \quad W = H\sqrt{\frac{6GB_3}{B_2^2 - 3B_1B_3}}. \quad \text{[S39]}$$

At this point it is also important to point out that the strain distribution defined by Eq. S38 exists only if $\Delta\varepsilon$, $W$ and $\varepsilon_{p1}$ are real valued, a condition that is satisfied only if

$$B_2^2 - 3B_3 > 0, \quad \text{and} \quad G > 0. \quad \text{[S40]}$$

Moreover, an explicit expression for the propagation stress can be obtained by substituting Eq. S39 into Eq. S36

$$\sigma_p = \sigma(\varepsilon_{p1}) = \frac{2B_2^3 - 9B_1B_2B_3}{27B_3^2}. \quad \text{[S41]}$$

and the position of the transition zone $Z_0$ is determined by introducing Eq. S38 into Eq. S35

$$\bar{\varepsilon} = \varepsilon_{p1} + \frac{\Delta\varepsilon}{2} + \frac{W\Delta\varepsilon}{Z_q - Z_p}\left\{\log\left[\cosh\left(\frac{Z_q - Z_0}{W}\right)\right] - \log\left[\cosh\left(\frac{Z_p - Z_0}{W}\right)\right]\right\}. \quad \text{[S42]}$$

Finally, we note that, since the energy barrier $\mathcal{S}_1$ is given by

$$\mathcal{S}_1 = \int_{\varepsilon_{p1}}^{\varepsilon_{p2}} (B_1\varepsilon_i + B_2\varepsilon_i^2 + B_3\varepsilon_i^3)\mathrm{d}\varepsilon_i - \sigma_p(\varepsilon_{p2} - \varepsilon_{p1}) = \frac{(B_2^2 - 3B_1B_3)^2}{36B_3^3}, \quad \text{[S43]}$$

where $\varepsilon_{pi}$ (with $i = 1$, 2 and 3) denote the three roots of

$$B_1\varepsilon + B_2\varepsilon^2 + B_3\varepsilon^3 = \sigma_p, \quad \text{[S44]}$$

the width of the transition zone can be expressed as,

$$W = \sqrt{\frac{G}{\sqrt{B_3\mathcal{S}_1}}}. \quad \text{[S45]}$$

Eq. S45 clearly show that the width of the transition zone $W$ is determined by the balance between $G$ (which captures the level of coupling between the unit cells) and $\mathcal{S}_1$ (which represent the energy barrier to overcome for the pop-up process to propagate). The larger is the coupling or the smaller is the energy barrier, the larger is the width of the transition zone.

### Movie S1. Propagation of instability in a long party balloon.

During inflation a long party balloon, first expands diametrically in a uniform fashion. However, at some value of pressure, the deformation localizes near an imperfection forming a bulge. Finally, as more compressed gas is made available, the bulge grows to a well defined diameter and then stops growing diametrically and starts growing in length. Inflation of a long party balloon is an example of instability propagation.

### Movie S2. Fabrication of kirigami shells.

Fabrication of a kirigami shell: ($i$) the double-sided adhesive is laser cut into the desired shape; ($ii$) the polyester sheet is attached to the adhesive layer and the kirigami pattern is laser cut; ($iii$) very thin adhesive black markers are attached to the sheet to track the deformation during testing; ($iv$) the two edges of the sheet are attached together using needles to facilitate alignment; ($v$) two bolted acrylic caps are laser cut; ($vi$) the caps are glued to the cylinder ends.

### Movie S3. Kirigami with triangular cuts: tensile response of sheet vs shell

Comparison between tensile deformation of three kirigami structures with triangular cuts: (left) a flat kirigami sheet characterized by $2 \times 20$ units with $\delta/l = 0.0625$, (middle) a kirigami shell characterized by $8 \times 20$ units with $\delta/l = 0.0333$ and (right) a kirigami shell characterized by $8 \times 20$ units with $\delta/l = 0.0625$. For all samples $t = 76.2\,\mu$m and $l = 12$ mm. The kirigami sheet and the kirigami shell with $\delta/l = 0.0333$ pop up uniformly while the kirigami shell with $\delta/l = 0.0625$ exhibits a propagating pop-up deformation. Dashed squares shows the magnified regions.

### Movie S4. Snapping propagation of pop-ups in a kirigami shell with triangular cuts.

Tensile response of a kirigami shell with triangular cuts characterized by $8 \times 20$ units with $\delta/l = 0.125$, $t = 76.2\,\mu$m and $l = 12$ mm. This structure is characterized by a large energy barrier $\mathcal{S}_1$, resulting in a sharp propagation front. As a result, the stress-strain curve of the structure is characterized by a discrete sequence of drops during propagation, each corresponding to the opening of one row of cuts. Dashed square shows the magnified region.

### Movie S5. Kirigami with linear cuts: tensile response of sheet vs shell

Comparison between tensile deformation of three kirigami structures with linear cuts: (left) a flat kirigami sheet with $3 \times 60$ units, (middle) a kirigami shell with $4 \times 60$ units and (right) a kirigami shell with $20 \times 60$ units. For all samples $\delta/l = 0.2$, $t = 76.2\,\mu$m and $l = 12$ mm. The kirigami sheet and the kirigami shell with $n = 4$ pop up uniformly, whereas the kirigami shell with $n = 20$ exhibits a propagative instability. Dashed squares shows the magnified regions.

### Movie S6. Kirigami with orthogonal cuts: tensile response of sheet vs shell

Comparison between tensile deformation of three kirigami structures with orthogonal cuts: (left) a flat kirigami sheet with $2 \times 20$ units, (middle) a kirigami shell with $4 \times 20$ units and (right) a kirigami shell with $20 \times 20$ units. For all samples $\delta/l = 0.08$, $t = 76.2\,\mu$m and $l = 6$ mm. The kirigami sheet and the kirigami shell with $n = 4$ pop up uniformly, whereas the kirigami shell with $n = 20$ exhibits a propagative instability. Dashed squares shows the magnified regions.

### Movie S7. Finite element simulations

(1) Deformation of unit cells of three kirigami structures with triangular cuts up to $\bar{\varepsilon} = 0.3$: (left) flat, (middle) initially curved, (right) rolled unit cells characterized by $n = 8$, $\delta/l = 0.0625$, $t = 76.2\,\mu$m and $l = 12$ mm. The contours show the distribution of the *von Mises* stress.

(2) Comparison between deformation of two kirigami shells with triangular cuts characterized by $\delta/l = 0.0625$ and $\delta/l = 0.125$ with $n = 8$, $t = 76.2\mu$ m and $l = 12$ mm. For each case the response of the unit cell, super cell and visually tessellated super cell are shown. The contours show the distribution of the *von Mise*s stress.

(3) Deformation of a kirigami shell with linear cuts characterized by $n = 20$, $\delta/l = 0.2$, $t = 76.2\,\mu$m and $l = 12$ mm: (left) unit cell, (middle) super cell and (right) visually tessellated super cell. The contours show the distribution of the *von Mises* stress.

(4) Deformation of a kirigami shell with orthogonal cuts characterized by $n = 20$, $\delta/l = 0.08$, $t = 76.2\,\mu$m and $l = 20$ mm: (left) unit cell, (middle) super cell and (right) visually tessellated super cell. The contours show the distribution of the *von Mises* stress.

### Movie S8. Programming pop-ups

(1) Response of programmed kirigami sheet and kirigami shell under tension. These kirigami surfaces comprise an array of triangular cuts separated by ligaments with width $\delta/l = 0.125$ in the center and $\delta/l = 0.033$ near the two two ends.

(2) Performance of three crawlers skinned with kirigami shells which exhibit uniform, propagating and programmed pop-up.

### Movie S9. Effect of imperfection

Deformation of an imperfect kirigami shells with triangular cuts which is characterized by $\delta/l = 0.125$ (with $l = 12$ mm) and $n = 8$. An imperfection is introduced in the middle of the shell by decreasing the width of one row of hinges to $\delta/l = 0.0625$.

## References


1. Abaqus, V., 2014. 6.14 Documentation. Dassault Systemes Simulia Corporation.
2. T.C. Shyu et *al* (2015). A kirigami approach to engineering elasticity in nanocomposites through patterned defects, *Nat Mat* 14:785–789.
3. A. Lamoureux, K. Lee, M. Shlian, S.R. Forrest, and M. Shtein (2015), Dynamic kirigami structures for integrated solar tracking, *Nat Commun* 6:8092.
4. M. Isobe and K. Okumura (2016), Initial rigid response and softening transition of highly stretchable kirigami sheet materials, *Sci Rep* 6:24758.
5. A. Rafsanjani and K. Bertoldi (2017), Buckling-induced Kirigami, *Phys Rev Lett* 118:084301.
6. A. Rafsanjani, Y. Zhang, B. Liu, S.M. Rubinstein and K. Bertoldi (2018), Kirigami skins make a simple soft actuator crawl, *Sci Robotics* 3(15):eaar7555.
7. M. Senn, C. Eberl, Digital Image Correlation and Tracking (2015). Available from: https://uk.mathworks.com/matlabcentral/fileexchange/50994-digital-image-correlation-and-tracking.
8. D. Polyzos, and D.I. Fotiadis (2012), Derivation of Mindlin's first and second strain gradient elastic theory via simple lattice and continuum models, *Int J Solids Struct* 49:470-480.
9. R.D. Mindlin (1964), Micro-structure in linear elasticity, *Arch Ration Mech Anal* 16:51-78.
10. J.C. Maxwell (1875), On the dynamical evidence of the molecular constitution of bodies, *Nature* 11:357-359.
11. M. Danielsson, D.M. Parks, M.C. Boyce (2002), Three-dimensional micromechanical modeling of voided polymeric materials, *J Mech Phys Solids* 50:351-379.
12. A. Polyanin, V. Zaitsev, Handbook of nonlinear partial differential equations (Chapman and Hall/CRC, London, 2011).
13. T. Dauxois, M. Peyrard, Physics of solitons (Cambridge University Press, London, 2006).
